# Supplementary material for: A comparison between short GRB afterglows and AT2017gfo: shedding light on kilonovae properties
Source: arXiv:1901.05792 source file (2020-01-14)
Supplement: Supplementary file 1 [file additional_figures_and_online_tables.pdf]

## Online material

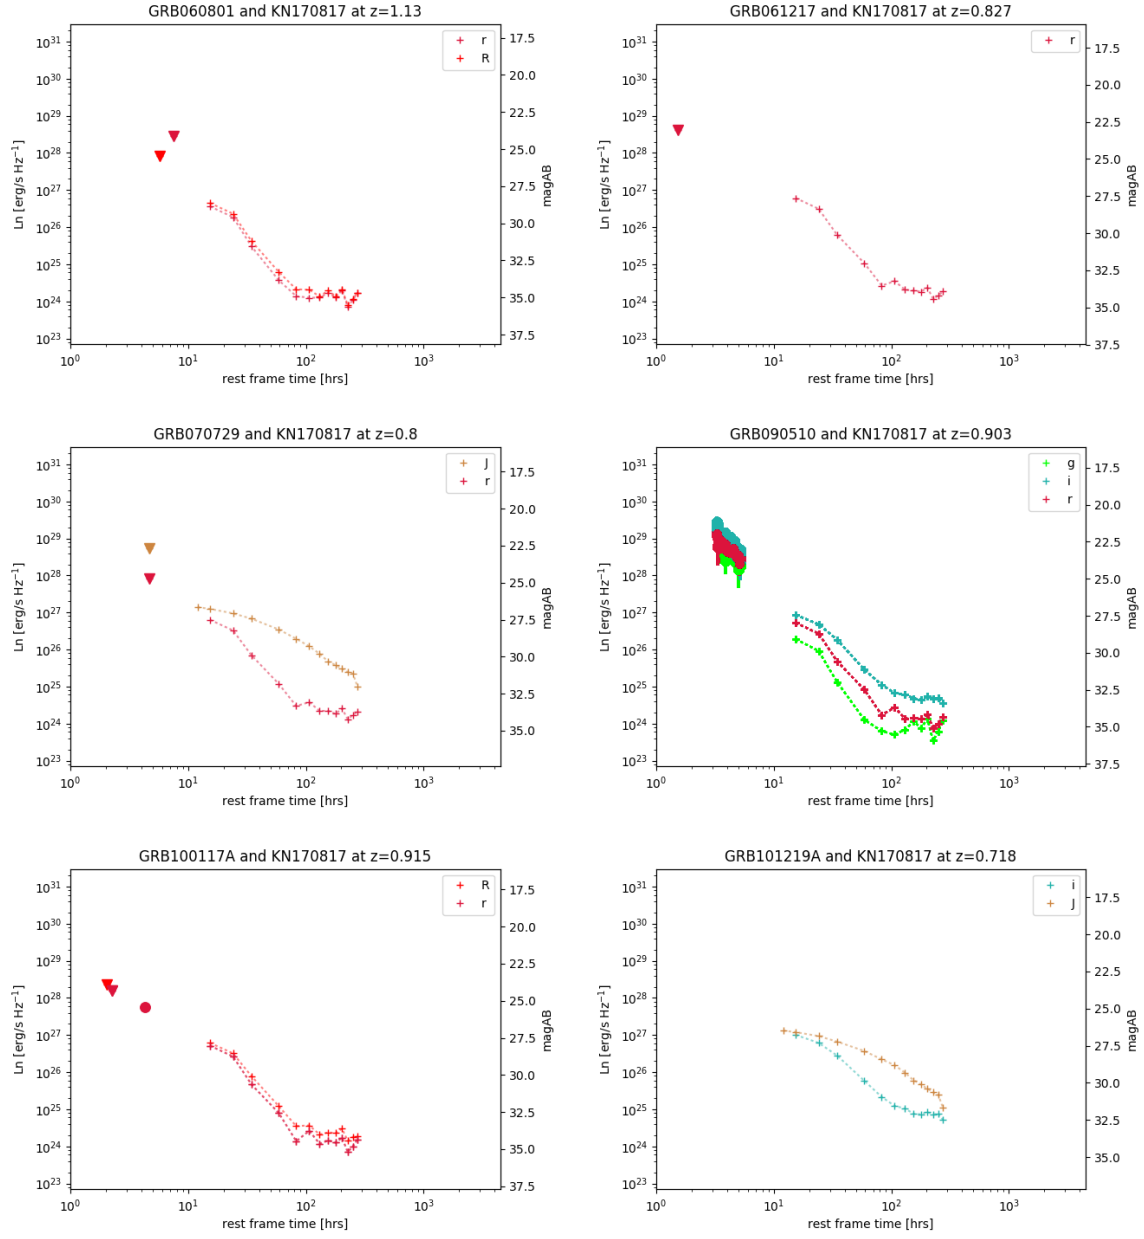

**Figure 1.** Short GRBs for which no optical data fall within the AT2017gfo sampled temporal window.

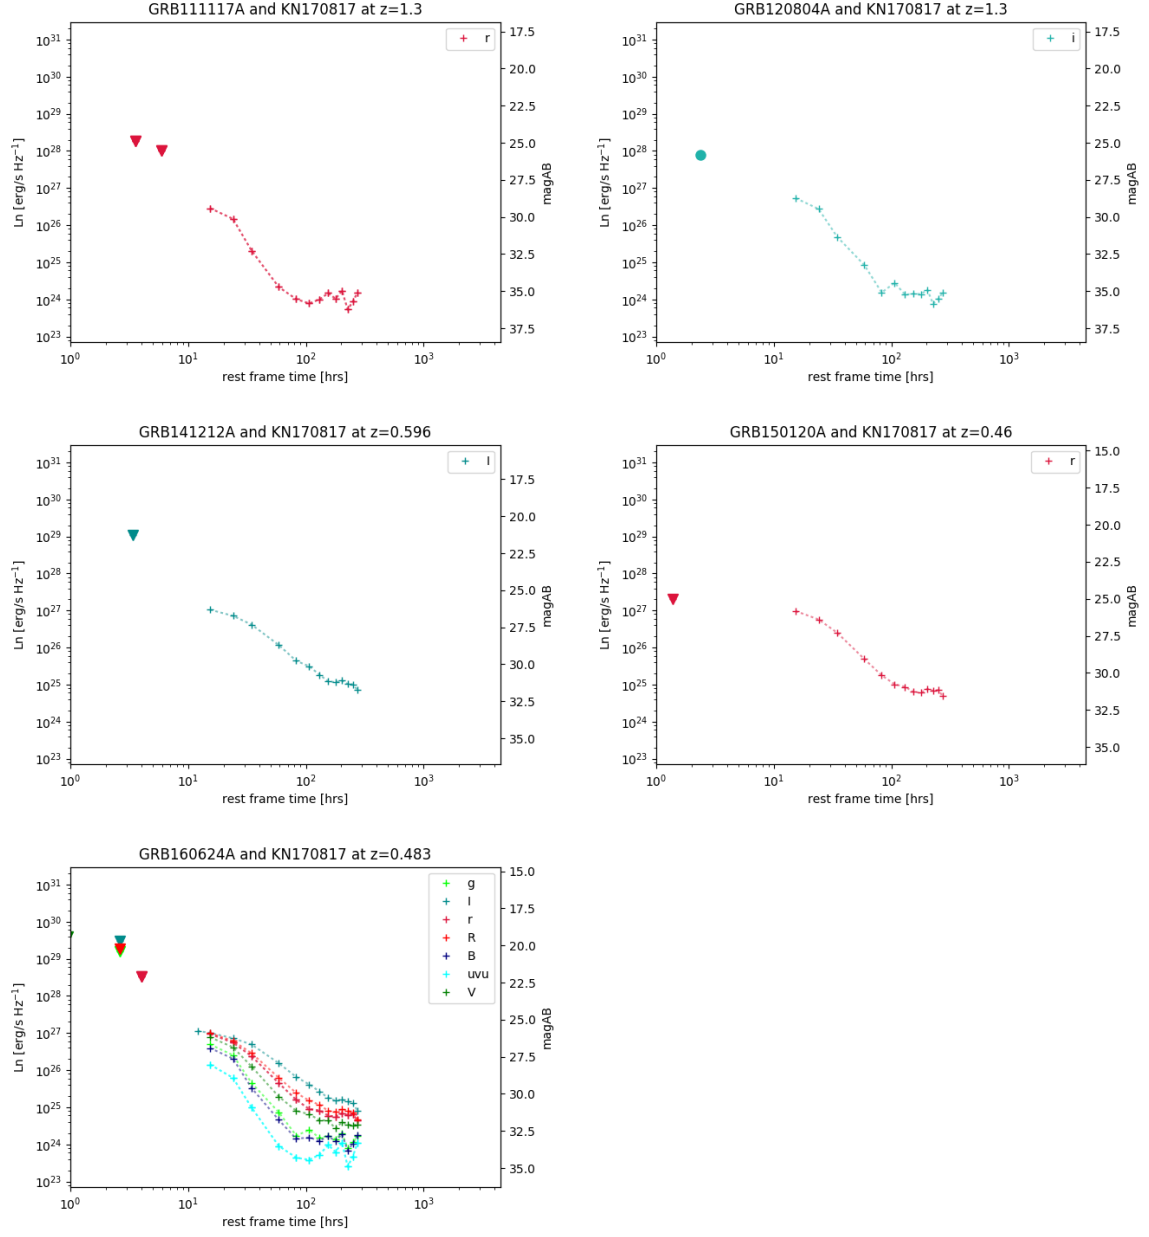

Figure 1 – continued

Table 1: Table with GRB and AT2017gfo luminosity ratios

| GRB     | time<br>hr | Band<br>eff. | $L_{GRB}$<br>$10^{26}$ erg/s Hz $^{-1}$ | $L_{KN}$<br>$10^{26}$ erg/s Hz $^{-1}$ | $L_{GRB}/L_{kn}$ | z     | $\lambda_{rest}$<br>nm | $\lambda_{obs}$<br>nm |
|---------|------------|--------------|-----------------------------------------|----------------------------------------|------------------|-------|------------------------|-----------------------|
| 050509B | 40.9       | g            | < 3.21                                  | 1.24                                   | < 2.59           | 0.225 | 391.7                  | 479.8                 |
| 050509B | 77.1       | V            | < 0.50                                  | 0.36                                   | < 1.38           | 0.225 | 454.9                  | 557.1                 |
| 050509B | 155.6      | V            | < 5.01                                  | 0.08                                   | < 59.43          | 0.225 | 454.9                  | 557.1                 |
| 050509B | 233.0      | V            | < 10.50                                 | 0.08                                   | < 123.82         | 0.225 | 454.9                  | 557.1                 |
| 050509B | 16.1       | R            | < 60.60                                 | 10.50                                  | < 5.77           | 0.225 | 523.5                  | 641.2                 |
| 050509B | 21.2       | R            | < 2.62                                  | 8.58                                   | < 0.31           | 0.225 | 523.5                  | 641.2                 |
| 050509B | 36.6       | R            | < 0.96                                  | 4.50                                   | < 0.21           | 0.225 | 523.5                  | 641.2                 |
| 050509B | 40.9       | R            | < 7.22                                  | 3.91                                   | < 1.85           | 0.225 | 523.5                  | 641.2                 |
| 050509B | 52.2       | R            | < 1.67                                  | 2.39                                   | < 0.70           | 0.225 | 523.5                  | 641.2                 |
| 050509B | 156.9      | R            | < 4.55                                  | 0.17                                   | < 26.76          | 0.225 | 523.5                  | 641.2                 |
| 050509B | 191.9      | I            | < 57.10                                 | 0.29                                   | < 194.22         | 0.225 | 645.5                  | 790.6                 |
| 050509B | 16.4       | J            | < 68.70                                 | 9.65                                   | < 7.12           | 0.225 | 1023.5                 | 1253.5                |
| 050509B | 34.1       | J            | < 157.00                                | 8.23                                   | < 19.08          | 0.225 | 1023.5                 | 1253.5                |
| 050509B | 132.7      | J            | < 43.30                                 | 2.89                                   | < 14.98          | 0.225 | 1023.5                 | 1253.5                |
| 050509B | 172.3      | J            | < 27.30                                 | 1.38                                   | < 19.78          | 0.225 | 1023.5                 | 1253.5                |
| 050509B | 14.2       | H            | < 110.00                                | 9.37                                   | < 11.74          | 0.225 | 1348.3                 | 1651.5                |
| 050509B | 18.4       | H            | < 83.70                                 | 9.39                                   | < 8.91           | 0.225 | 1348.3                 | 1651.5                |
| 050509B | 73.4       | H            | < 101.00                                | 6.80                                   | < 14.85          | 0.225 | 1348.3                 | 1651.5                |
| 050509B | 15.8       | K            | < 262.00                                | 7.88                                   | < 33.25          | 0.225 | 1764.6                 | 2161.2                |
| 050709  | 38.2       | V            | < 53.60                                 | 3.17                                   | < 16.91          | 0.161 | 480.0                  | 557.1                 |
| 050709  | 50.9       | V            | $4.17 \pm 0.46$                         | 1.78                                   | 2.34             | 0.161 | 480.0                  | 557.1                 |
| 050709  | 90.2       | V            | < 2.34                                  | 0.29                                   | < 7.96           | 0.161 | 480.0                  | 557.1                 |
| 050709  | 216.8      | V            | < 3.89                                  | 0.11                                   | < 35.36          | 0.161 | 480.0                  | 557.1                 |
| 050709  | 23.7       | R            | < 82.20                                 | 7.87                                   | < 10.44          | 0.161 | 552.5                  | 641.2                 |
| 050709  | 24.5       | R            | < 327.00                                | 7.64                                   | < 42.80          | 0.161 | 552.5                  | 641.2                 |
| 050709  | 25.5       | R            | < 47.30                                 | 7.40                                   | < 6.39           | 0.161 | 552.5                  | 641.2                 |
| 050709  | 29.3       | R            | $15.20 \pm 0.78$                        | 6.51                                   | 2.33             | 0.161 | 552.5                  | 641.2                 |
| 050709  | 51.1       | R            | $5.86 \pm 0.33$                         | 2.91                                   | 2.01             | 0.161 | 552.5                  | 641.2                 |
| 050709  | 51.7       | R            | $7.62 \pm 1.69$                         | 2.83                                   | 2.69             | 0.161 | 552.5                  | 641.2                 |
| 050709  | 137.4      | R            | < 1.43                                  | 0.27                                   | < 5.28           | 0.161 | 552.5                  | 641.2                 |
| 050709  | 152.6      | R            | < 4.73                                  | 0.21                                   | < 22.96          | 0.161 | 552.5                  | 641.2                 |
| 050709  | 173.2      | R            | < 47.30                                 | 0.18                                   | < 259.89         | 0.161 | 552.5                  | 641.2                 |
| 050709  | 216.7      | R            | < 2.98                                  | 0.16                                   | < 18.74          | 0.161 | 552.5                  | 641.2                 |
| 050709  | 25.6       | i            | < 155.00                                | 8.66                                   | < 17.90          | 0.161 | 659.6                  | 765.5                 |
| 050709  | 50.8       | I            | $3.73 \pm 0.75$                         | 4.50                                   | 0.83             | 0.161 | 681.2                  | 790.6                 |
| 050709  | 90.4       | I            | < 3.73                                  | 1.67                                   | < 2.23           | 0.161 | 681.2                  | 790.6                 |
| 050709  | 115.8      | I            | $2.21 \pm 0.04$                         | 1.03                                   | 2.15             | 0.161 | 681.2                  | 790.6                 |
| 050709  | 172.3      | I            | < 1.96                                  | 0.40                                   | < 4.84           | 0.161 | 681.2                  | 790.6                 |
| 050709  | 202.6      | I            | $1.11 \pm 0.05$                         | 0.32                                   | 3.48             | 0.161 | 681.2                  | 790.6                 |
| 050709  | 116.7      | K            | $6.24 \pm 5.65$                         | 6.28                                   | 0.99             | 0.161 | 1862.2                 | 2161.2                |
| 050724  | 66.1       | V            | < 18.00                                 | 0.49                                   | < 36.51          | 0.258 | 442.9                  | 557.1                 |
| 050724  | 27.8       | R            | $57.80 \pm 5.00$                        | 6.38                                   | 9.06             | 0.258 | 509.7                  | 641.2                 |
| 050724  | 46.7       | R            | < 27.90                                 | 2.92                                   | < 9.55           | 0.258 | 509.7                  | 641.2                 |
| 050724  | 65.8       | R            | < 19.30                                 | 1.12                                   | < 17.23          | 0.258 | 509.7                  | 641.2                 |
| 050724  | 27.7       | I            | $48.50 \pm 5.69$                        | 8.07                                   | 6.01             | 0.258 | 628.5                  | 790.6                 |
| 050724  | 29.2       | I            | < 157.00                                | 7.73                                   | < 20.31          | 0.258 | 628.5                  | 790.6                 |
| 050724  | 66.1       | I            | $5.69 \pm 2.07$                         | 2.34                                   | 2.43             | 0.258 | 628.5                  | 790.6                 |
| 050724  | 27.7       | K            | < 93.10                                 | 7.93                                   | < 11.74          | 0.258 | 1718.0                 | 2161.2                |
| 051221A | 17.4       | r            | $203.00 \pm 15.50$                      | 7.93                                   | 25.60            | 0.546 | 404.8                  | 625.9                 |
| 051221A | 33.4       | r            | $75.60 \pm 8.95$                        | 2.34                                   | 32.31            | 0.546 | 404.8                  | 625.9                 |
| 051221A | 49.0       | r            | $76.50 \pm 22.80$                       | 1.00                                   | 76.50            | 0.546 | 404.8                  | 625.9                 |
| 051221A | 80.0       | r            | $40.70 \pm 8.95$                        | 0.15                                   | 276.87           | 0.546 | 404.8                  | 625.9                 |
| 051221A | 95.6       | r            | < 26.00                                 | 0.10                                   | < 273.40         | 0.546 | 404.8                  | 625.9                 |
| 051221A | 17.6       | i            | $187.00 \pm 43.90$                      | 9.86                                   | 18.97            | 0.546 | 495.2                  | 765.5                 |

Continued on next page

Table 1 – continued from previous page

|         |       |   |                     |       |           |       |        |        |
|---------|-------|---|---------------------|-------|-----------|-------|--------|--------|
| 051221A | 33.0  | i | $67.50 \pm 26.00$   | 4.31  | 15.66     | 0.546 | 495.2  | 765.5  |
| 051221A | 33.2  | z | $89.50 \pm 38.20$   | 5.78  | 15.48     | 0.546 | 581.2  | 898.5  |
| 060502B | 31.7  | r | < 11.50             | 4.63  | < 2.48    | 0.287 | 486.3  | 625.9  |
| 060614  | 19.8  | V | $179.00 \pm 57.00$  | 8.93  | 20.04     | 0.125 | 495.2  | 557.1  |
| 060614  | 12.8  | R | $240.00 \pm 48.50$  | 11.90 | 20.17     | 0.125 | 569.9  | 641.2  |
| 060614  | 38.0  | R | $60.20 \pm 19.20$   | 5.04  | 11.94     | 0.125 | 569.9  | 641.2  |
| 060614  | 13.8  | I | $271.00 \pm 26.20$  | 12.90 | 21.01     | 0.125 | 702.8  | 790.6  |
| 060614  | 13.8  | J | $326.00 \pm 31.40$  | 9.60  | 33.96     | 0.125 | 1114.3 | 1253.5 |
| 061006  | 34.6  | R | $77.40 \pm 8.78$    | 3.20  | 24.19     | 0.438 | 446.0  | 641.2  |
| 061006  | 31.9  | I | $129.00 \pm 8.78$   | 5.76  | 22.40     | 0.438 | 549.9  | 790.6  |
| 061006  | 41.7  | I | $134.00 \pm 11.40$  | 4.18  | 32.06     | 0.438 | 549.9  | 790.6  |
| 061201  | 29.8  | I | < 2.76              | 7.97  | < 0.35    | 0.111 | 711.6  | 790.6  |
| 061201  | 73.3  | I | < 1.91              | 2.74  | < 0.70    | 0.111 | 711.6  | 790.6  |
| 061210  | 48.7  | R | $653.00 \pm 132.00$ | 1.89  | 345.50    | 0.410 | 454.7  | 641.2  |
| 070429B | 14.2  | J | < 900.00            | 13.10 | < 68.70   | 0.902 | 659.1  | 1253.5 |
| 070714B | 54.9  | R | $60.20 \pm 19.20$   | 0.23  | 262.88    | 0.923 | 333.4  | 641.2  |
| 070714B | 12.5  | J | < 2140.00           | 13.90 | < 153.96  | 0.923 | 651.9  | 1253.5 |
| 070714B | 12.5  | K | $647.00 \pm 206.00$ | 9.51  | 68.03     | 0.923 | 1123.9 | 2161.2 |
| 070724A | 14.7  | I | < 272.00            | 10.40 | < 26.15   | 0.456 | 543.0  | 790.6  |
| 070724A | 47.0  | I | < 235.00            | 3.32  | < 70.78   | 0.456 | 543.0  | 790.6  |
| 070724A | 81.0  | I | < 257.00            | 0.76  | < 336.83  | 0.456 | 543.0  | 790.6  |
| 070724A | 114.1 | I | < 246.00            | 0.39  | < 622.78  | 0.456 | 543.0  | 790.6  |
| 070724A | 163.3 | I | < 742.00            | 0.17  | < 4364.71 | 0.456 | 543.0  | 790.6  |
| 070724A | 229.1 | I | < 293.00            | 0.13  | < 2253.85 | 0.456 | 543.0  | 790.6  |
| 070724A | 14.7  | J | < 482.00            | 9.55  | < 50.47   | 0.456 | 861.0  | 1253.5 |
| 070724A | 47.0  | J | < 428.00            | 5.72  | < 74.83   | 0.456 | 861.0  | 1253.5 |
| 070724A | 81.0  | J | < 1940.00           | 2.78  | < 697.84  | 0.456 | 861.0  | 1253.5 |
| 070724A | 114.1 | J | < 1470.00           | 1.96  | < 750.00  | 0.456 | 861.0  | 1253.5 |
| 070724A | 163.3 | J | < 954.00            | 0.92  | < 1034.71 | 0.456 | 861.0  | 1253.5 |
| 070724A | 229.2 | J | < 902.00            | 0.40  | < 2243.78 | 0.456 | 861.0  | 1253.5 |
| 070724A | 18.6  | K | < 3850.00           | 9.00  | < 427.78  | 0.456 | 1484.4 | 2161.2 |
| 070809  | 23.9  | g | < 11.50             | 2.65  | < 4.34    | 0.473 | 325.7  | 479.8  |
| 070809  | 23.8  | R | $21.80 \pm 6.66$    | 6.32  | 3.45      | 0.473 | 435.3  | 641.2  |
| 071227  | 21.0  | g | < 9.41              | 4.22  | < 2.23    | 0.381 | 347.4  | 479.8  |
| 071227  | 21.0  | r | < 14.80             | 7.85  | < 1.89    | 0.381 | 453.2  | 625.9  |
| 071227  | 21.0  | i | < 30.70             | 8.18  | < 3.75    | 0.381 | 554.3  | 765.5  |
| 071227  | 21.0  | z | < 25.40             | 10.10 | < 2.51    | 0.381 | 650.6  | 898.5  |
| 071227  | 21.0  | J | < 365.00            | 8.96  | < 40.74   | 0.381 | 907.7  | 1253.5 |
| 071227  | 21.0  | H | < 913.00            | 9.75  | < 93.64   | 0.381 | 1195.8 | 1651.5 |
| 080905A | 15.6  | r | < 13.60             | 9.98  | < 1.36    | 0.122 | 557.9  | 625.9  |
| 080905A | 12.8  | R | $3.49 \pm 1.15$     | 11.90 | 0.29      | 0.122 | 571.6  | 641.2  |
| 080905A | 32.1  | R | < 1.77              | 6.14  | < 0.29    | 0.122 | 571.6  | 641.2  |
| 080905A | 15.6  | J | < 101.00            | 9.70  | < 10.41   | 0.122 | 1117.5 | 1253.5 |
| 090515  | 17.8  | r | $4.00 \pm 1.43$     | 9.10  | 0.44      | 0.403 | 446.1  | 625.9  |
| 100625A | 23.4  | J | < 55.10             | 8.65  | < 6.37    | 0.452 | 863.3  | 1253.5 |
| 100816A | 26.6  | r | $79.50 \pm 16.10$   | 2.64  | 30.11     | 0.805 | 346.8  | 625.9  |
| 100816A | 53.2  | r | $66.10 \pm 13.40$   | 0.24  | 269.80    | 0.805 | 346.8  | 625.9  |
| 130603B | 28.2  | g | < 6.39              | 2.38  | < 2.68    | 0.356 | 353.8  | 479.8  |
| 130603B | 23.0  | r | < 10.10             | 7.14  | < 1.41    | 0.356 | 461.6  | 625.9  |
| 130603B | 23.8  | r | < 15.50             | 6.82  | < 2.27    | 0.356 | 461.6  | 625.9  |
| 130603B | 28.3  | r | $7.06 \pm 1.68$     | 5.28  | 1.34      | 0.356 | 461.6  | 625.9  |
| 130603B | 23.0  | i | < 19.50             | 7.59  | < 2.57    | 0.356 | 564.6  | 765.5  |
| 130603B | 28.5  | i | < 16.10             | 6.35  | < 2.54    | 0.356 | 564.6  | 765.5  |
| 130603B | 28.5  | J | < 121.00            | 8.54  | < 14.17   | 0.356 | 924.4  | 1253.5 |
| 130603B | 164.7 | H | $5.71 \pm 1.01$     | 1.88  | 3.04      | 0.356 | 1217.9 | 1651.5 |
| 140903A | 27.5  | r | < 430.00            | 5.57  | < 77.20   | 0.351 | 463.3  | 625.9  |
| 140903A | 44.4  | r | < 156.00            | 2.24  | < 69.64   | 0.351 | 463.3  | 625.9  |
| 140903A | 79.8  | r | < 89.90             | 0.34  | < 262.10  | 0.351 | 463.3  | 625.9  |
| 140903A | 29.0  | i | $81.40 \pm 10.40$   | 6.27  | 12.98     | 0.351 | 566.6  | 765.5  |

Continued on next page

Table 1 – continued from previous page

|         |       |     |                    |       |             |       |        |        |
|---------|-------|-----|--------------------|-------|-------------|-------|--------|--------|
| 150101B | 35.1  | r   | $10.10 \pm 1.52$   | 4.86  | 2.08        | 0.134 | 551.9  | 625.9  |
| 150101B | 56.1  | r   | $6.25 \pm 1.70$    | 1.96  | 3.19        | 0.134 | 551.9  | 625.9  |
| 150101B | 226.6 | r   | < 3.39             | 0.14  | < 24.04     | 0.134 | 551.9  | 625.9  |
| 150101B | 203.7 | J   | < 33.90            | 1.05  | < 32.29     | 0.134 | 1105.4 | 1253.5 |
| 150423A | 90.2  | z   | < 7840.00          | 0.07  | < 114956.00 | 1.394 | 375.3  | 898.5  |
| 150424A | 21.2  | uvu | < 379.00           | 1.87  | < 202.67    | 0.300 | 266.4  | 346.3  |
| 150424A | 39.7  | uvu | < 456.00           | 0.17  | < 2698.22   | 0.300 | 266.4  | 346.3  |
| 150424A | 169.9 | uvu | < 288.00           | 0.01  | < 23801.70  | 0.300 | 266.4  | 346.3  |
| 150424A | 27.6  | B   | < 494.00           | 2.28  | < 216.67    | 0.300 | 335.2  | 435.8  |
| 150424A | 33.4  | g   | $43.90 \pm 4.23$   | 1.42  | 30.92       | 0.300 | 369.1  | 479.8  |
| 150424A | 51.0  | g   | < 33.90            | 0.47  | < 71.97     | 0.300 | 369.1  | 479.8  |
| 150424A | 69.1  | g   | < 14.80            | 0.12  | < 118.40    | 0.300 | 369.1  | 479.8  |
| 150424A | 88.0  | g   | < 10.20            | 0.06  | < 175.86    | 0.300 | 369.1  | 479.8  |
| 150424A | 124.6 | g   | < 40.80            | 0.04  | < 1108.70   | 0.300 | 369.1  | 479.8  |
| 150424A | 143.3 | g   | < 25.70            | 0.03  | < 823.72    | 0.300 | 369.1  | 479.8  |
| 150424A | 180.1 | g   | < 19.50            | 0.03  | < 693.95    | 0.300 | 369.1  | 479.8  |
| 150424A | 34.4  | V   | < 1010.00          | 2.59  | < 389.96    | 0.300 | 428.5  | 557.1  |
| 150424A | 16.4  | r   | $157.00 \pm 16.70$ | 10.30 | 15.24       | 0.300 | 481.4  | 625.9  |
| 150424A | 33.5  | r   | $53.80 \pm 3.58$   | 3.98  | 13.52       | 0.300 | 481.4  | 625.9  |
| 150424A | 51.0  | r   | < 15.90            | 1.78  | < 8.93      | 0.300 | 481.4  | 625.9  |
| 150424A | 69.1  | r   | $24.80 \pm 5.57$   | 0.68  | 36.63       | 0.300 | 481.4  | 625.9  |
| 150424A | 88.0  | r   | < 9.18             | 0.32  | < 28.51     | 0.300 | 481.4  | 625.9  |
| 150424A | 122.5 | r   | $3.56 \pm 0.20$    | 0.17  | 20.34       | 0.300 | 481.4  | 625.9  |
| 150424A | 124.6 | r   | < 25.30            | 0.17  | < 148.82    | 0.300 | 481.4  | 625.9  |
| 150424A | 143.3 | r   | < 21.00            | 0.13  | < 165.35    | 0.300 | 481.4  | 625.9  |
| 150424A | 170.3 | r   | $1.48 \pm 0.20$    | 0.10  | 14.51       | 0.300 | 481.4  | 625.9  |
| 150424A | 180.1 | r   | < 14.50            | 0.10  | < 142.16    | 0.300 | 481.4  | 625.9  |
| 150424A | 256.0 | r   | $0.56 \pm 0.23$    | 0.09  | 6.46        | 0.300 | 481.4  | 625.9  |
| 150424A | 12.4  | i   | $239.00 \pm 11.30$ | 11.30 | 21.15       | 0.300 | 588.9  | 765.5  |
| 150424A | 13.4  | i   | $241.00 \pm 9.04$  | 11.00 | 21.91       | 0.300 | 588.9  | 765.5  |
| 150424A | 14.4  | i   | $212.00 \pm 9.98$  | 10.60 | 20.00       | 0.300 | 588.9  | 765.5  |
| 150424A | 16.4  | i   | $199.00 \pm 17.20$ | 9.91  | 20.08       | 0.300 | 588.9  | 765.5  |
| 150424A | 33.5  | i   | $55.70 \pm 7.09$   | 5.72  | 9.74        | 0.300 | 588.9  | 765.5  |
| 150424A | 51.0  | i   | < 25.00            | 3.07  | < 8.14      | 0.300 | 588.9  | 765.5  |
| 150424A | 69.1  | i   | < 20.80            | 1.45  | < 14.34     | 0.300 | 588.9  | 765.5  |
| 150424A | 88.0  | i   | < 13.10            | 0.76  | < 17.15     | 0.300 | 588.9  | 765.5  |
| 150424A | 124.6 | i   | < 33.00            | 0.37  | < 88.71     | 0.300 | 588.9  | 765.5  |
| 150424A | 143.3 | i   | < 27.40            | 0.26  | < 105.39    | 0.300 | 588.9  | 765.5  |
| 150424A | 180.1 | i   | < 17.30            | 0.19  | < 92.02     | 0.300 | 588.9  | 765.5  |
| 150424A | 12.4  | z   | $274.00 \pm 15.60$ | 14.00 | 19.57       | 0.300 | 691.2  | 898.5  |
| 150424A | 13.4  | z   | $247.00 \pm 11.70$ | 13.50 | 18.30       | 0.300 | 691.2  | 898.5  |
| 150424A | 14.4  | z   | $222.00 \pm 12.60$ | 13.00 | 17.08       | 0.300 | 691.2  | 898.5  |
| 150424A | 16.4  | z   | < 767.00           | 12.20 | < 62.87     | 0.300 | 691.2  | 898.5  |
| 150424A | 33.4  | z   | $80.40 \pm 9.40$   | 7.09  | 11.34       | 0.300 | 691.2  | 898.5  |
| 150424A | 51.0  | z   | < 32.60            | 4.43  | < 7.36      | 0.300 | 691.2  | 898.5  |
| 150424A | 69.1  | z   | < 27.10            | 2.67  | < 10.15     | 0.300 | 691.2  | 898.5  |
| 150424A | 88.0  | z   | < 15.60            | 1.65  | < 9.45      | 0.300 | 691.2  | 898.5  |
| 150424A | 124.6 | z   | < 43.00            | 0.81  | < 53.09     | 0.300 | 691.2  | 898.5  |
| 150424A | 143.3 | z   | < 56.70            | 0.56  | < 100.35    | 0.300 | 691.2  | 898.5  |
| 150424A | 180.1 | z   | < 22.60            | 0.35  | < 63.84     | 0.300 | 691.2  | 898.5  |
| 150424A | 12.4  | J   | $361.00 \pm 69.00$ | 9.36  | 38.57       | 0.300 | 964.3  | 1253.5 |
| 150424A | 13.4  | J   | $289.00 \pm 55.30$ | 9.38  | 30.81       | 0.300 | 964.3  | 1253.5 |
| 150424A | 14.4  | J   | $250.00 \pm 58.90$ | 9.40  | 26.60       | 0.300 | 964.3  | 1253.5 |
| 150424A | 33.5  | J   | < 129.00           | 8.25  | < 15.64     | 0.300 | 964.3  | 1253.5 |
| 150424A | 51.0  | J   | < 141.00           | 6.65  | < 21.20     | 0.300 | 964.3  | 1253.5 |
| 150424A | 69.1  | J   | < 155.00           | 5.02  | < 30.88     | 0.300 | 964.3  | 1253.5 |
| 150424A | 88.0  | J   | < 97.60            | 3.64  | < 26.81     | 0.300 | 964.3  | 1253.5 |
| 150424A | 123.2 | J   | $7.06 \pm 0.54$    | 2.49  | 2.84        | 0.300 | 964.3  | 1253.5 |
| 150424A | 123.7 | J   | $6.75 \pm 0.00$    | 2.47  | 2.73        | 0.300 | 964.3  | 1253.5 |

Continued on next page

Table 1 – continued from previous page

|         |       |   |                 |       |          |       |        |        |
|---------|-------|---|-----------------|-------|----------|-------|--------|--------|
| 150424A | 143.4 | J | < 129.00        | 1.77  | < 72.88  | 0.300 | 964.3  | 1253.5 |
| 150424A | 171.0 | J | $2.64 \pm 0.56$ | 1.15  | 2.30     | 0.300 | 964.3  | 1253.5 |
| 150424A | 180.1 | J | < 97.60         | 1.00  | < 97.60  | 0.300 | 964.3  | 1253.5 |
| 150424A | 256.6 | J | $1.55 \pm 0.00$ | 0.39  | 4.02     | 0.300 | 964.3  | 1253.5 |
| 150424A | 257.1 | J | $1.31 \pm 0.62$ | 0.38  | 3.43     | 0.300 | 964.3  | 1253.5 |
| 150424A | 33.5  | H | < 203.00        | 7.84  | < 25.89  | 0.300 | 1270.3 | 1651.5 |
| 150424A | 51.0  | H | < 203.00        | 7.41  | < 27.40  | 0.300 | 1270.3 | 1651.5 |
| 150424A | 69.1  | H | < 222.00        | 6.45  | < 34.42  | 0.300 | 1270.3 | 1651.5 |
| 150424A | 88.0  | H | < 140.00        | 5.12  | < 27.34  | 0.300 | 1270.3 | 1651.5 |
| 150424A | 123.9 | H | $8.19 \pm 0.54$ | 3.62  | 2.26     | 0.300 | 1270.3 | 1651.5 |
| 150424A | 143.4 | H | < 203.00        | 2.64  | < 76.89  | 0.300 | 1270.3 | 1651.5 |
| 150424A | 171.7 | H | $4.10 \pm 0.56$ | 1.67  | 2.46     | 0.300 | 1270.3 | 1651.5 |
| 150424A | 180.1 | H | < 185.00        | 1.48  | < 125.00 | 0.300 | 1270.3 | 1651.5 |
| 150424A | 257.8 | H | $1.27 \pm 0.64$ | 0.49  | 2.59     | 0.300 | 1270.3 | 1651.5 |
| 150424A | 33.5  | K | < 557.00        | 7.00  | < 79.57  | 0.300 | 1662.5 | 2161.2 |
| 150424A | 51.0  | K | < 882.00        | 7.73  | < 114.10 | 0.300 | 1662.5 | 2161.2 |
| 150424A | 69.1  | K | < 967.00        | 7.27  | < 133.01 | 0.300 | 1662.5 | 2161.2 |
| 150424A | 88.0  | K | < 610.00        | 5.94  | < 102.69 | 0.300 | 1662.5 | 2161.2 |
| 150424A | 143.4 | K | < 557.00        | 3.67  | < 151.77 | 0.300 | 1662.5 | 2161.2 |
| 150424A | 180.2 | K | < 385.00        | 2.33  | < 165.24 | 0.300 | 1662.5 | 2161.2 |
| 160821B | 74.5  | r | $1.19 \pm 0.38$ | 0.89  | 1.34     | 0.160 | 539.5  | 625.9  |
| 160821B | 75.4  | r | $0.99 \pm 0.04$ | 0.85  | 1.16     | 0.160 | 539.5  | 625.9  |
| 160821B | 215.1 | r | $0.16 \pm 0.05$ | 0.13  | 1.19     | 0.160 | 539.5  | 625.9  |
| 160821B | 78.1  | J | $2.96 \pm 0.08$ | 6.06  | 0.49     | 0.160 | 1080.7 | 1253.5 |
| 160821B | 217.8 | J | $0.51 \pm 0.10$ | 0.76  | 0.66     | 0.160 | 1080.7 | 1253.5 |
| 160821B | 76.7  | H | $3.81 \pm 0.14$ | 6.76  | 0.56     | 0.160 | 1423.7 | 1651.5 |
| 160821B | 216.4 | H | $0.42 \pm 0.13$ | 1.12  | 0.37     | 0.160 | 1423.7 | 1651.5 |
| 160821B | 102.8 | K | $5.82 \pm 2.36$ | 6.77  | 0.86     | 0.160 | 1863.2 | 2161.2 |
| 160821B | 169.0 | K | < 5.93          | 3.36  | < 1.76   | 0.160 | 1863.2 | 2161.2 |
| 160821B | 187.6 | K | < 6.93          | 2.65  | < 2.62   | 0.160 | 1863.2 | 2161.2 |
| 170428A | 17.5  | r | < 260.00        | 8.75  | < 29.71  | 0.454 | 430.4  | 625.9  |
| 170428A | 17.5  | Y | < 1210.00       | 11.80 | < 102.54 | 0.454 | 617.9  | 898.5  |
| 170428A | 17.5  | z | < 924.00        | 10.60 | < 87.17  | 0.454 | 617.9  | 898.5  |
| 170428A | 17.5  | J | < 1910.00       | 9.24  | < 206.71 | 0.454 | 862.1  | 1253.5 |
| 170428A | 17.5  | H | < 2290.00       | 9.79  | < 233.91 | 0.454 | 1135.8 | 1651.5 |

Table 2: Short GRBs with known redshift in addition to [Fong et al. \(2015\)](#)

| GRB     | $\Delta T$<br>hours | Telescope/Instr      | Filter  | mag              | Flux density<br>$\mu Jy$ | Gal. Ext.<br>$A_V$ | Refs                                 |
|---------|---------------------|----------------------|---------|------------------|--------------------------|--------------------|--------------------------------------|
| 130603B | 700                 | HST                  | F160W   | > 26.90          | < 0.07                   | 0.06               | <a href="#">Tanvir et al. (2013)</a> |
| 160410A | 0.533               | ESO/MPG GROND        | g       | 20.60 $\pm$ 0.10 | 21.89 $\pm$ 2.11         | 0.02               | GCN#19272                            |
|         | 0.533               | ESO/MPG GROND        | r       | 20.50 $\pm$ 0.10 | 23.86 $\pm$ 2.30         |                    |                                      |
|         | 0.533               | ESO/MPG GROND        | i       | 20.70 $\pm$ 0.10 | 19.76 $\pm$ 1.91         |                    |                                      |
|         | 0.533               | ESO/MPG GROND        | z       | 20.50 $\pm$ 0.20 | 23.67 $\pm$ 4.79         |                    |                                      |
|         | 0.533               | ESO/MPG GROND        | J       | > 20.00          | < 37.39                  |                    |                                      |
|         | 0.533               | ESO/MPG GROND        | H       | > 19.60          | < 53.93                  |                    |                                      |
|         | 0.533               | ESO/MPG GROND        | Ks      | > 18.00          | < 235.2                  |                    |                                      |
|         | 0.128               | ESO/VLT X-shooter    | r       | 20.29 $\pm$ 0.06 | 28.95 $\pm$ 1.65         |                    | GCN#19274                            |
|         | 0.0253              | Swift/UVOT           | uvwhite | 19.46 $\pm$ 0.10 | 30.39 $\pm$ 2.93         |                    | GCN#19275                            |
|         | 1.3519              | Swift/UVOT           | uvv     | > 19.70          | < 49.09                  |                    |                                      |
|         | 1.1808              | Swift/UVOT           | uvb     | > 20.20          | < 34.49                  |                    |                                      |
|         | 0.0844              | Swift/UVOT           | uvu     | 20.50 $\pm$ 0.20 | 9.90 $\pm$ 2.00          |                    |                                      |
|         | 1.4658              | Swift/UVOT           | uvw1    | > 20.30          | < 6.79                   |                    |                                      |
|         | 1.4089              | Swift/UVOT           | uvm2    | > 20.80          | < 3.31                   |                    |                                      |
|         | 1.295               | Swift/UVOT           | uvw2    | > 20.50          | < 4.16                   |                    |                                      |
|         | 0.0167              | Skynet/CTIO PROMPT   | I       | 17.30 $\pm$ 0.30 | 301.0 $\pm$ 95.8         |                    | GCN#19277                            |
|         | 0.1                 | Skynet/CTIO PROMPT   | I       | 19.40 $\pm$ 0.30 | 43.50 $\pm$ 13.84        |                    |                                      |
|         | 7.5                 | GMC 2.4-m OT         | R       | 22.10 $\pm$ 0.20 | 4.58 $\pm$ 0.93          |                    | GCN#19280                            |
|         | 7.1                 | MITSuME 3colorCCDcam | g       | > 19.80          | < 45.74                  |                    | GCN#19285                            |
|         | 7.1                 | MITSuME 3colorCCDcam | Rc      | > 19.70          | < 41.05                  |                    |                                      |
|         | 7.1                 | MITSuME 3colorCCDcam | I       | > 19.10          | < 57.35                  |                    |                                      |
|         | 0.0078              | ESO/TAROT            | R       | 18.40 $\pm$ 0.30 | 138.30 $\pm$ 44.02       |                    | GCN#19287                            |
|         | 0.0128              | ESO/TAROT            | R       | > 18.70          | < 104.9                  |                    |                                      |
|         | 0.0244              | ESO/TAROT            | R       | > 18.70          | < 104.9                  |                    |                                      |
|         | 25.3                | UKIRT WFCAM          | J       | > 20.00          | < 37.39                  |                    | GCN#19290                            |
|         | 25.3                | UKIRT WFCAM          | K       | > 19.50          | < 59.07                  |                    |                                      |
|         | 17.3                | NOT ALFOSC           | r       | 24.15 $\pm$ 0.09 | 0.83 $\pm$ 0.07          |                    | GCN#19295                            |
|         | 40.37               | NOT ALFOSC           | r       | > 25.00          | < 0.38                   |                    | GCN#19300                            |
|         | 14.6                | TLS                  | I       | > 21.10          | < 13.63                  |                    | GCN#19309                            |
|         | 20.7                | CTIO ANDICAM         | I       | > 20.30          | < 18.99                  |                    | GCN#19311                            |
|         | 20.7                | CTIO ANDICAM         | J       | > 17.50          | < 158.8                  |                    |                                      |
| 150423A | 0.4                 | ESO/MPG GROND        | g       | 23.20 $\pm$ 0.20 | 2.01 $\pm$ 0.41          | 0.03               | GCN#17729                            |
|         | 0.4                 | ESO/MPG GROND        | r       | 23.10 $\pm$ 0.20 | 2.19 $\pm$ 0.44          |                    |                                      |
|         | 0.4                 | ESO/MPG GROND        | i       | 22.50 $\pm$ 0.20 | 3.78 $\pm$ 0.77          |                    |                                      |
|         | 0.4                 | ESO/MPG GROND        | z       | 22.00 $\pm$ 0.20 | 5.97 $\pm$ 1.21          |                    |                                      |
|         | 0.4                 | ESO/MPG GROND        | J       | 19.30 $\pm$ 0.40 | 71.40 $\pm$ 31.80        |                    |                                      |
|         | 0.4                 | ESO/MPG GROND        | H       | > 18.40          | < 163.1                  |                    |                                      |
|         | 0.4                 | ESO/MPG GROND        | Ks      | > 17.50          | < 373.1                  |                    |                                      |
|         | 0.0322              | KAIT                 | R       | > 17.00          | < 504.9                  |                    | GCN#19730                            |
|         | 0.9667              | ESO/MPG GROND        | g       | 23.20 $\pm$ 0.20 | 2.01 $\pm$ 0.41          |                    | GCN#17732                            |
|         | 0.9667              | ESO/MPG GROND        | r       | 23.10 $\pm$ 0.20 | 2.19 $\pm$ 0.44          |                    |                                      |
|         | 0.9667              | ESO/MPG GROND        | i       | 22.80 $\pm$ 0.20 | 2.87 $\pm$ 0.58          |                    |                                      |
|         | 0.9667              | ESO/MPG GROND        | z       | 22.60 $\pm$ 0.20 | 3.43 $\pm$ 0.69          |                    |                                      |
|         | 0.9667              | ESO/MPG GROND        | J       | > 21.60          | < 8.58                   |                    |                                      |
|         | 0.9667              | ESO/MPG GROND        | H       | > 21.00          | < 14.87                  |                    |                                      |
|         | 0.9667              | ESO/MPG GROND        | Ks      | > 18.50          | < 148.5                  |                    |                                      |
|         | 4.155               | JOHNSON RATIR        | r       | 23.77 $\pm$ 0.23 | 1.18 $\pm$ 0.28          |                    | GCN#17736                            |
|         | 4.155               | JOHNSON RATIR        | i       | 23.62 $\pm$ 0.26 | 1.35 $\pm$ 0.36          |                    |                                      |
|         | 4.155               | JOHNSON RATIR        | Zg      | > 20.33          | < 27.76                  |                    |                                      |
|         | 1.5667              | ESO/VLT FORS2        | Rc      | 22.80 $\pm$ 0.10 | 2.38 $\pm$ 0.23          |                    | GCN#17738                            |
|         | 0.0205              | Swift/UVOT           | uvwhite | > 20.80          | < 8.97                   |                    | GCN#17739                            |
|         | 0.0794              | Swift/UVOT           | uvu     | > 20.20          | < 13.19                  |                    |                                      |

Continued on next page

Table 2 – continued from previous page

|         |         |                         |         |             |              |                     |
|---------|---------|-------------------------|---------|-------------|--------------|---------------------|
|         | 0.0205  | Swift/UVOT              | uvwhite | > 21.50     | < 4.71       |                     |
|         | 0.1708  | Swift/UVOT              | uvv     | > 20.90     | <16.37       |                     |
|         | 0.1503  | Swift/UVOT              | uvb     | > 20.90     | <18.28       |                     |
|         | 0.0794  | Swift/UVOT              | uvu     | > 20.80     | <7.59        |                     |
|         | 0.1847  | Swift/UVOT              | uvw1    | > 20.90     | <3.97        |                     |
|         | 1.4022  | Swift/UVOT              | uvm2    | > 20.80     | <3.38        |                     |
|         | 0.1642  | Swift/UVOT              | uvw2    | > 21.60     | <1.54        |                     |
|         | 10.6    | MITSuME 3colorCCDcam    | g       | > 20.80     | <18.37       | GCN#17742           |
|         | 10.6    | MITSuME 3colorCCDcam    | Rc      | > 20.80     | <14.99       |                     |
|         | 10.6    | MITSuME 3colorCCDcam    | I       | > 19.90     | < 27.54      |                     |
|         | 16.0344 | WHT ACAM                | g       | >25.30      | <0.29        | GCN#17747           |
|         | 0.5756  | Zeiss-1000-East 1-m tel | R       | >22.70      | <2.65        | GCN#17750           |
|         | 25.355  | JOHNSON RATIR           | r       | > 24.82     | <0.45        | GCN#17754           |
|         | 25.355  | JOHNSON RATIR           | i       | > 24.79     | <0.46        |                     |
|         | 25.355  | JOHNSON RATIR           | Zg      | > 22.07     | <5.59        |                     |
|         | 6.6     | MITSuME 3colorCCDcam    | g       | > 19.4      | < 66.68      | GCN#17763           |
|         | 6.6     | MITSuME 3colorCCDcam    | Rc      | > 19.3      | <59.69       |                     |
|         | 6.6     | MITSuME 3colorCCDcam    | I       | > 18.4      | <109.7       |                     |
|         | 216     | GMC 2.4-m OT            | z       | >21.00      | <14.99       | GCN#17803           |
| 160624A | 0.7667  | Gemini North GMOS-N     | r       | >25.50      | <0.25        | 0.07 GCN#19565 (AG) |
|         | 3.9     | MITSuME 3colorCCDcam    | g       | > 20.50     | <25.34       | GCN#19571           |
|         | 3.9     | MITSuME 3colorCCDcam    | Rc      | > 20.10     | < 29.49      |                     |
|         | 3.9     | MITSuME 3colorCCDcam    | I       | > 19.30     | < 48.78      |                     |
|         | 6       | 1-m Lulin               | r       | > 22.20     | < 5.18       | GCN#19575           |
|         | 0.0214  | Swift/UVOT              | uvwhite | > 20.80     | <9.66        | GCN#19576           |
|         | 0.0802  | Swift/UVOT              | uvu     | > 20.00     | <16.84       |                     |
|         | 0.0214  | Swift/UVOT              | uvwhite | > 21.50     | < 5.07       |                     |
|         | 1.4056  | Swift/UVOT              | uvv     | > 19.50     | < 61.82      |                     |
|         | 1.2347  | Swift/UVOT              | uvb     | > 20.70     | < 23.14      |                     |
|         | 0.0802  | Swift/UVOT              | uvu     | > 20.70     | < 8.84       |                     |
|         | 1.5197  | Swift/UVOT              | uvw1    | > 20.80     | < 4.72       |                     |
|         | 1.4628  | Swift/UVOT              | uvm2    | > 20.70     | < 4.16       |                     |
|         | 1.3486  | Swift/UVOT              | uvw2    | > 20.30     | < 5.61       |                     |
| 170428A | 10.16   | 2.16-m Xinglong         | R       | > 21.00     | < 12.95      | 0.06 GCN#21048      |
|         | 0.2056  | Swift/UVOT              | uvv     | > 20.00     | < 38.57      | GCN#21049           |
|         | 0.2328  | Swift/UVOT              | uvb     | > 21.00     | < 17.29      |                     |
|         | 0.2258  | Swift/UVOT              | uvu     | > 19.50     | < 26.23      |                     |
|         | 0.2192  | Swift/UVOT              | uvw1    | > 19.50     | < 15.25      |                     |
|         | 0.2122  | Swift/UVOT              | uvm2    | > 20.10     | < 6.98       |                     |
|         | 1.22    | Swift/UVOT              | uvw2    | > 20.00     | < 7.19       |                     |
|         | 1.0667  | ESO/MPG GROND           | g       | 21.40± 0.10 | 10.91± 1.05  | GCN#21050           |
|         | 1.0667  | ESO/MPG GROND           | r       | 21.30± 0.10 | 11.76± 1.14  |                     |
|         | 1.0667  | ESO/MPG GROND           | i       | 21.10± 0.10 | 13.98± 1.35  |                     |
|         | 1.0667  | ESO/MPG GROND           | z       | 21.10± 0.10 | 13.84± 1.34  |                     |
|         | 1.0667  | ESO/MPG GROND           | J       | 20.70± 0.20 | 19.82± 4.01  |                     |
|         | 1.0667  | ESO/MPG GROND           | H       | 20.90± 0.40 | 16.39± 7.30  |                     |
|         | 1.0667  | ESO/MPG GROND           | Ks      | >20.00      | < 37.43      |                     |
|         | 25.47   | JOHNSON RATIR           | r       | >22.30      | <4.68        | GCN#21051           |
|         | 25.47   | JOHNSON RATIR           | Zg      | >20.90      | <16.62       |                     |
|         | 25.47   | JOHNSON RATIR           | Y       | >20.60      | <21.85       |                     |
|         | 25.47   | JOHNSON RATIR           | J       | >20.10      | <34.44       |                     |
|         | 25.47   | JOHNSON RATIR           | H       | >19.90      | <41.16       |                     |
|         | 0.0153  | ESO/TAROT               | R       | > 17.50     | <325.3       | GCN#21052           |
|         | 0.0314  | ESO/TAROT               | R       | > 18.20     | <170.7       |                     |
|         | 0.0675  | ESO/TAROT               | R       | > 19.20     | <67.96       |                     |
| 150424A | 1.6     | Keck I LRIS             | R       | 20.00± 0.30 | 32.52± 10.35 | 0.06 GCN#17745      |
|         | 13.2    | NOT/ALFOSC              | R       | 20.67± 0.06 | 17.55± 1.00  | GCN#17756           |
|         | 15.54   | ESO/MPG GROND           | g       | 22.00±0.20  | 6.28± 1.27   | GCN#17757           |
|         | 15.54   | ESO/MPG GROND           | r       | 21.60± 0.10 | 8.92± 0.86   |                     |

Continued on next page

Table 2 – continued from previous page

|         |               |                |             |              |                     |
|---------|---------------|----------------|-------------|--------------|---------------------|
| 15.54   | ESO/MPG GROND | i              | 21.40± 0.10 | 10.61± 1.02  |                     |
| 15.54   | ESO/MPG GROND | z              | 21.10± 0.10 | 13.84± 1.34  |                     |
| 15.54   | ESO/MPG GROND | J              | 20.40± 0.50 | 26.12± 15.28 |                     |
| 15.54   | ESO/MPG GROND | H              | > 19.90     | <41.16       |                     |
| 21.295  | JOHNSON RATIR | r              | 21.92± 0.11 | 6.64± 0.71   | GCN#17762           |
| 21.295  | JOHNSON RATIR | i              | 21.65± 0.09 | 8.43± 0.73   | GCN#17761           |
| 21.295  | JOHNSON RATIR | Z <sub>g</sub> | > 20.17     | < 32.55      |                     |
| 160.8   | HST           | J              | >25.30      | <0.29        | GCN#18100           |
| 333.6   | HST           | J              | >26.90      | <0.07        |                     |
| 16.0842 | ESO/MPG GROND | g              | 21.76± 0.04 | 7.83± 0.29   | Knust et al. (2017) |
| 17.4014 | ESO/MPG GROND | g              | 21.90± 0.03 | 6.89±0.19    |                     |
| 18.6881 | ESO/MPG GROND | g              | 21.99± 0.04 | 6.34±0.24    |                     |
| 43.3675 | ESO/MPG GROND | g              | 23.32± 0.10 | 1.86±0.18    |                     |
| 66.3611 | ESO/MPG GROND | g              | > 23.60     | < 1.44       |                     |
| 89.7828 | ESO/MPG GROND | g              | > 24.50     | <0.63        |                     |
| 114.38  | ESO/MPG GROND | g              | > 24.90     | < 0.43       |                     |
| 161.938 | ESO/MPG GROND | g              | > 23.40     | < 1.73       |                     |
| 186.296 | ESO/MPG GROND | g              | > 23.90     | <1.09        |                     |
| 234.094 | ESO/MPG GROND | g              | > 24.20     | < 0.83       |                     |
| 16.0842 | ESO/MPG GROND | r              | 21.55± 0.03 | 9.34± 0.26   |                     |
| 17.4014 | ESO/MPG GROND | r              | 21.60± 0.03 | 8.92± 0.25   |                     |
| 18.6881 | ESO/MPG GROND | r              | 21.80± 0.03 | 7.42± 0.21   |                     |
| 43.495  | ESO/MPG GROND | r              | 23.08± 0.07 | 2.28± 0.15   |                     |
| 66.3611 | ESO/MPG GROND | r              | > 24.40     | <0.68        |                     |
| 89.7828 | ESO/MPG GROND | r              | 23.92± 0.22 | 1.05± 0.24   |                     |
| 114.38  | ESO/MPG GROND | r              | >25.00      | < 0.39       |                     |
| 161.938 | ESO/MPG GROND | r              | > 23.90     | < 1.07       |                     |
| 186.359 | ESO/MPG GROND | r              | > 24.10     | < 0.89       |                     |
| 234.156 | ESO/MPG GROND | r              | > 24.50     | < 0.62       |                     |
| 16.0842 | ESO/MPG GROND | i              | 21.45± 0.05 | 10.14± 0.48  |                     |
| 17.4014 | ESO/MPG GROND | i              | 21.44± 0.04 | 10.23± 0.38  |                     |
| 18.715  | ESO/MPG GROND | i              | 21.58± 0.05 | 8.99± 0.42   |                     |
| 43.495  | ESO/MPG GROND | i              | 23.03± 0.13 | 2.37± 0.30   |                     |
| 66.3611 | ESO/MPG GROND | i              | > 23.90     | < 1.06       |                     |
| 89.7828 | ESO/MPG GROND | i              | > 24.10     | < 0.88       |                     |
| 114.38  | ESO/MPG GROND | i              | > 24.60     | < 0.56       |                     |
| 161.938 | ESO/MPG GROND | i              | > 23.60     | < 1.40       |                     |
| 186.359 | ESO/MPG GROND | i              | > 23.80     | < 1.16       |                     |
| 234.156 | ESO/MPG GROND | i              | > 24.30     | <0.73        |                     |
| 16.0842 | ESO/MPG GROND | z              | 21.29± 0.06 | 11.63± 0.66  |                     |
| 17.4014 | ESO/MPG GROND | z              | 21.40± 0.05 | 10.58±0.49   |                     |
| 18.715  | ESO/MPG GROND | z              | 21.52± 0.06 | 9.400± 0.53  |                     |
| 43.4319 | ESO/MPG GROND | z              | 22.62± 0.12 | 3.414± 0.40  |                     |
| 66.3611 | ESO/MPG GROND | z              | > 23.60     | <1.39        |                     |
| 89.7828 | ESO/MPG GROND | z              | > 23.80     | < 1.15       |                     |
| 114.38  | ESO/MPG GROND | z              | > 24.40     | < 0.66       |                     |
| 161.938 | ESO/MPG GROND | z              | > 23.30     | < 1.83       |                     |
| 186.359 | ESO/MPG GROND | z              | > 23.00     | < 2.41       |                     |
| 234.156 | ESO/MPG GROND | z              | >24.00      | < 0.96       |                     |
| 16.0914 | ESO/MPG GROND | J              | 20.98± 0.19 | 15.32± 2.93  |                     |
| 17.4083 | ESO/MPG GROND | J              | 21.22± 0.19 | 12.29± 2.35  |                     |
| 18.7219 | ESO/MPG GROND | J              | 21.38± 0.23 | 10.60± 2.50  |                     |
| 43.5017 | ESO/MPG GROND | J              | >22.10      | < 5.46       |                     |
| 66.3678 | ESO/MPG GROND | J              | >22.00      | < 5.99       |                     |
| 89.8142 | ESO/MPG GROND | J              | >21.90      | < 6.56       |                     |
| 114.386 | ESO/MPG GROND | J              | > 22.40     | < 4.15       |                     |
| 186.365 | ESO/MPG GROND | J              | > 22.10     | < 5.46       |                     |
| 234.163 | ESO/MPG GROND | J              | > 22.40     | < 4.15       |                     |
| 43.5017 | ESO/MPG GROND | H              | > 21.60     | < 8.60       |                     |

Continued on next page

Table 2 – continued from previous page

|         |               |         |            |            |
|---------|---------------|---------|------------|------------|
| 66.3678 | ESO/MPG GROND | H       | > 21.60    | < 8.60     |
| 89.8142 | ESO/MPG GROND | H       | > 21.50    | < 9.43     |
| 114.386 | ESO/MPG GROND | H       | > 22.00    | < 5.95     |
| 186.365 | ESO/MPG GROND | H       | > 21.60    | < 8.60     |
| 234.163 | ESO/MPG GROND | H       | > 21.70    | < 7.84     |
| 43.565  | ESO/MPG GROND | Ks      | > 20.50    | < 23.63    |
| 66.3678 | ESO/MPG GROND | Ks      | > 20.00    | < 37.44    |
| 89.7894 | ESO/MPG GROND | Ks      | > 19.90    | < 41.05    |
| 114.386 | ESO/MPG GROND | Ks      | > 20.40    | < 25.98    |
| 186.365 | ESO/MPG GROND | Ks      | > 20.50    | < 23.63    |
| 234.289 | ESO/MPG GROND | Ks      | > 20.90    | < 16.35    |
| 0.1211  | Swift/UVOT    | uvu     | > 21.30    | <12.21     |
| 0.8019  | Swift/UVOT    | uvu     | > 20.80    | <19.35     |
| 1.7767  | Swift/UVOT    | uvu     | 20.56±0.23 | 24.14±5.60 |
| 0.9456  | Swift/UVOT    | uvu     | 20.91±0.17 | 17.49±2.96 |
| 12.6642 | Swift/UVOT    | uvu     | > 21.30    | <12.21     |
| 27.6    | Swift/UVOT    | uvu     | >21.00     | <16.10     |
| 51.5578 | Swift/UVOT    | uvu     | > 20.80    | <19.35     |
| 220.91  | Swift/UVOT    | uvu     | > 21.30    | <12.21     |
| 387.388 | Swift/UVOT    | uvu     | > 22.10    | <5.84      |
| 0.1844  | Swift/UVOT    | uvb     | > 18.90    | <110.1     |
| 1.6344  | Swift/UVOT    | uvb     | 20.42±0.25 | 27.15±7.03 |
| 1.0094  | Swift/UVOT    | uvb     | > 20.90    | <17.45     |
| 4.4906  | Swift/UVOT    | uvb     | > 20.50    | <25.22     |
| 4.4906  | Swift/UVOT    | uvb     | > 21.00    | <15.91     |
| 35.9467 | Swift/UVOT    | uvb     | > 20.70    | <20.98     |
| 0.0228  | Swift/UVOT    | vv      | > 17.50    | <392.8     |
| 0.205   | Swift/UVOT    | uvv     | > 18.00    | <247.8     |
| 1.2075  | Swift/UVOT    | uvv     | > 19.10    | <89.97     |
| 1.6061  | Swift/UVOT    | uvv     | > 19.60    | <56.77     |
| 0.9058  | Swift/UVOT    | uvv     | > 19.80    | <47.22     |
| 3.355   | Swift/UVOT    | uvv     | > 19.90    | <43.06     |
| 5.6375  | Swift/UVOT    | uvv     | > 20.10    | <35.82     |
| 9.6503  | Swift/UVOT    | uvv     | > 19.90    | <43.06     |
| 44.6922 | Swift/UVOT    | uvv     | > 19.90    | <43.06     |
| 0.7703  | Swift/UVOT    | uvw1    | > 20.90    | <18.16     |
| 4.9817  | Swift/UVOT    | uvw1    | 21.27±0.19 | 12.92±2.47 |
| 11.7344 | Swift/UVOT    | uvw1    | > 22.20    | <5.48      |
| 25.7381 | Swift/UVOT    | uvw1    | > 22.10    | <6.01      |
| 49.4342 | Swift/UVOT    | uvw1    | > 21.80    | <7.93      |
| 207.41  | Swift/UVOT    | uvw1    | > 22.40    | <4.56      |
| 364.036 | Swift/UVOT    | uvw1    | > 22.60    | <3.79      |
| 0.1983  | Swift/UVOT    | uvw2    | > 19.70    | <56.07     |
| 0.9303  | Swift/UVOT    | uvw2    | > 21.20    | <14.08     |
| 0.8739  | Swift/UVOT    | uvw2    | > 21.90    | <7.39      |
| 3.1444  | Swift/UVOT    | uvw2    | 21.65±0.17 | 9.31±1.58  |
| 8.1253  | Swift/UVOT    | uvw2    | 21.89±0.10 | 7.46±0.72  |
| 35.9161 | Swift/UVOT    | uvw2    | > 22.60    | <3.88      |
| 59.8933 | Swift/UVOT    | uvw2    | > 22.50    | <4.25      |
| 119.762 | Swift/UVOT    | uvw2    | > 23.10    | <2.45      |
| 359.838 | Swift/UVOT    | uvw2    | > 23.20    | <2.23      |
| 0.2117  | Swift/UVOT    | uvm2    | > 19.10    | <99.97     |
| 1.4636  | Swift/UVOT    | uvm2    | > 21.20    | <14.45     |
| 0.9378  | Swift/UVOT    | uvm2    | > 21.70    | <9.12      |
| 20.1128 | Swift/UVOT    | uvm2    | > 21.90    | <7.58      |
| 48.1072 | Swift/UVOT    | uvm2    | > 22.30    | <5.25      |
| 143.458 | Swift/UVOT    | uvm2    | > 22.50    | <4.36      |
| 340.146 | Swift/UVOT    | uvm2    | > 22.40    | <4.79      |
| 0.0483  | Swift/UVOT    | uvwhite | 21.30±0.23 | 12.46±2.94 |

Continued on next page

Table 2 – continued from previous page

|         |         |                            |         |             |                                 |      |                        |
|---------|---------|----------------------------|---------|-------------|---------------------------------|------|------------------------|
|         | 0.1669  | Swift/UVOT                 | uvwhite | >20.70      | <21.65                          |      |                        |
|         | 0.2472  | Swift/UVOT                 | uvwhite | 20.94±0.16  | 17.36±2.76                      |      |                        |
|         | 1.4919  | Swift/UVOT                 | uvwhite | 20.96±0.15  | 17.04±2.53                      |      |                        |
|         | 2.3558  | Swift/UVOT                 | uvwhite | 20.93±0.08  | 17.52±1.34                      |      |                        |
|         | 2.9342  | Swift/UVOT                 | uvwhite | 20.87±0.09  | 18.51±1.60                      |      |                        |
|         | 4.7017  | Swift/UVOT                 | uvwhite | 21.09±0.10  | 15.12±1.46                      |      |                        |
|         | 8.9239  | Swift/UVOT                 | uvwhite | 21.02±0.06  | 16.12±0.92                      |      |                        |
|         | 81.2894 | Swift/UVOT                 | uvwhite | > 22.80     | <3.13                           |      |                        |
|         | 84.4175 | Swift/UVOT                 | uvwhite | > 22.70     | <3.43                           |      |                        |
|         | 87.4589 | Swift/UVOT                 | uvwhite | > 22.20     | <5.44                           |      |                        |
|         | 93.2061 | Swift/UVOT                 | uvwhite | > 22.30     | <4.96                           |      |                        |
|         | 99.7006 | Swift/UVOT                 | uvwhite | > 22.60     | <3.76                           |      |                        |
|         | 1.5567  | Keck I LRIS                | g       | 20.77±0.03  | 19.49± 0.55                     |      |                        |
|         | 1.56    | Keck I LRIS                | Rc      | 20.66±0.04  | 21.16±0.79                      |      |                        |
|         | 159.286 | HST WFC3                   | F606W   | 26.03±0.06  | (151.10±8.59)×10 <sup>-3</sup>  |      | Jin et al. (2018)      |
|         | 221.363 | HST WFC3                   | F606W   | 26.98±0.14  | (62.99±8.67)×10 <sup>-3</sup>   |      |                        |
|         | 332.847 | HST WFC3                   | F606W   | 28.03±0.37  | (23.95±9.72)×10 <sup>-3</sup>   |      |                        |
|         | 160.206 | HST WFC3                   | F125W   | 25.25±0.08  | (299.70±22.92)×10 <sup>-3</sup> |      |                        |
|         | 222.324 | HST WFC3                   | F125W   | 26.32±0.21  | (111.90±23.87)×10 <sup>-3</sup> |      |                        |
|         | 334.199 | HST WFC3                   | F125W   | 27.08±0.42  | (55.60±26.24)×10 <sup>-3</sup>  |      |                        |
|         | 161.017 | HST WFC3                   | F160W   | 25.08±0.07  | (347.40±23.14)×10 <sup>-3</sup> |      |                        |
|         | 223.177 | HST WFC3                   | F160W   | 25.83±0.14  | (174.10±23.97)×10 <sup>-3</sup> |      |                        |
|         | 335.073 | HST WFC3                   | F160W   | 27.10±0.44  | (54.06±27.01)×10 <sup>-3</sup>  |      |                        |
| 160821B | 119.207 | Keck I MOSFIRE             | Ks      | 24.04±0.37  | 0.90±0.37                       | 0.04 | Kasliwal et al. (2017) |
|         | 196.008 | Keck I MOSFIRE             | Ks      | >24.02      | <0.92                           |      |                        |
|         | 217.608 | Keck I MOSFIRE             | Ks      | >23.85      | <1.08                           |      |                        |
|         | 0.95    | NOT ALFOSC                 | R       | 22.60±0.10  | 2.94±0.28                       |      | GCN#19834              |
|         | 0.0211  | Swift/UVOT                 | uvwhite | >21.10      | <6.98                           |      | GCN#19839              |
|         | 0.08    | Swift/UVOT                 | uvu     | >20.40      | <11.20                          |      |                        |
|         | 0.0211  | Swift/UVOT                 | uvwhite | >21.70      | <4.02                           |      |                        |
|         | 1.4111  | Swift/UVOT                 | uvv     | >19.10      | <87.08                          |      |                        |
|         | 1.6392  | Swift/UVOT                 | uvb     | >20.20      | <35.44                          |      |                        |
|         | 0.08    | Swift/UVOT                 | uvu     | >20.60      | <9.32                           |      |                        |
|         | 1.5253  | Swift/UVOT                 | uvw1    | >19.60      | <13.50                          |      |                        |
|         | 1.4681  | Swift/UVOT                 | uvm2    | >19.50      | <11.63                          |      |                        |
|         | 1.3542  | Swift/UVOT                 | uvw2    | >20.10      | <6.33                           |      |                        |
|         | 1.83    | GTC OSIRIS                 | R       | 22.40±0.06  | 3.53±0.20                       |      | GCN#19847              |
|         | 86.4    | HST WFC3                   | F606W   | 25.80±0.30  | (18.44±5.87)×10 <sup>-2</sup>   |      | GCN#20222              |
|         | 87.45   | HST WFC3                   | F606W   | 26.00±0.04  | (15.34±0.58)×10 <sup>-2</sup>   |      | Jin et al. (2018)      |
|         | 249.508 | HST WFC3                   | F606W   | 28.00±0.30  | (2.43±0.77)×10 <sup>-2</sup>    |      |                        |
|         | 555.844 | HST WFC3                   | F606W   | >27.9       | <0.027                          |      |                        |
|         | 90.5954 | HST WFC3                   | F110W   | 24.78±0.03  | (46.09±1.29)×10 <sup>-2</sup>   |      |                        |
|         | 252.654 | HST WFC3                   | F110W   | 26.70±0.20  | (7.86±1.59)×10 <sup>-2</sup>    |      |                        |
|         | 556.341 | HST WFC3                   | F110W   | > 28.00     | <0.024                          |      |                        |
|         | 89.0066 | HST WFC3                   | F160W   | 24.50±0.04  | (59.19±2.22)×10 <sup>-2</sup>   |      |                        |
|         | 251.065 | HST WFC3                   | F160W   | 26.90±0.30  | (6.49±2.07)×10 <sup>-2</sup>    |      |                        |
|         | 557.53  | HST WFC3                   | F160W   | >27.00      | <0.059                          |      |                        |
| 060614  | 1.5981  | Swift/UVOT                 | uvu     | 19.54±0.30  | 25.21±8.02                      | 0.06 | GCN#5255               |
|         | 1.4286  | Swift/UVOT                 | uvb     | 19.91±0.21  | 47.07±10.04                     |      |                        |
|         | 1.3714  | Swift/UVOT                 | uvu     | 18.81±0.14  | 49.38±6.80                      |      |                        |
|         | 1.3139  | Swift/UVOT                 | uvw1    | 18.35±0.17  | 43.82±7.43                      |      |                        |
|         | 1.6553  | Swift/UVOT                 | uvw1    | 18.06±0.23  | 57.23±13.50                     |      |                        |
|         | 1.5422  | Swift/UVOT                 | uvw1    | 18.26±0.17  | 47.60±8.07                      |      |                        |
|         | 0.0408  | Swift/UVOT                 | uvwhite | 18.30±0.14  | 94.21±12.97                     |      |                        |
|         | 7.1     | Boydén Obs. Watcher 0.4m   | R       | 19.00±0.3 0 | 81.59±25.97                     |      | GCN#5257               |
|         | 0.4296  | Siding Spring Obs. 1m Tel. | R       | 20.20±0.30  | 27.02±8.60                      |      | GCN#5258               |
|         | 0.5304  | Siding Spring Obs. 1m Tel. | R       | 19.90±0.20  | 35.62±7.20                      |      |                        |
|         | 0.6288  | Siding Spring Obs. 1m Tel. | R       | 19.90±0.20  | 35.62±7.20                      |      |                        |
|         | 0.7272  | Siding Spring Obs. 1m Tel. | R       | 19.90±0.20  | 35.62±7.20                      |      |                        |

Continued on next page

Table 2 – continued from previous page

|         |         |                            |      |            |             |      |                                         |
|---------|---------|----------------------------|------|------------|-------------|------|-----------------------------------------|
|         | 1.7112  | Siding Spring Obs. 1m Tel. | R    | 19.10±0.10 | 74.41±7.18  |      |                                         |
|         | 2.8512  | Siding Spring Obs. 1m Tel. | R    | 19.20±0.10 | 67.87±6.55  |      |                                         |
|         | 3.8592  | Siding Spring Obs. 1m Tel. | R    | 19.10±0.10 | 74.41±7.18  |      |                                         |
|         | 4.7232  | Siding Spring Obs. 1m Tel. | R    | 19.00±0.10 | 81.59±7.87  |      |                                         |
|         | 5.8248  | Siding Spring Obs. 1m Tel. | R    | 18.80±0.10 | 98.10±9.46  |      |                                         |
|         | 15.5    | CTIO ANDICAM               | I    | 18.90±0.10 | 70.06±6.76  |      | GCN#5259                                |
|         | 15.5    | CTIO ANDICAM               | J    | 18.20±0.10 | 84.11±8.12  |      |                                         |
|         | 14.4    | ESO/VLT FORS2              | R    | 19.30±0.20 | 61.89±12.52 |      | GCN#5261                                |
|         | 22.2222 | Swift/UVOT                 | uvv  | 19.80±0.30 | 46.28±14.73 |      | GCN#5262                                |
|         | 42.72   | ESO/VLT FORS1              | R    | 20.80±0.30 | 15.55±4.95  |      | GCN#5271                                |
|         | 360     | Swift/UVOT                 | uvu  | >24.00     | <0.41       |      | GCN#5286                                |
| 080905A | 36      | VLT FORS2                  | R    | >25.00     | <0.48       | 0.37 | <a href="#">Rowlinson et al. (2010)</a> |
|         | 14.3    | VLT FORS2                  | R    | 24.26±0.31 | 0.95±0.31   |      |                                         |
|         | 8.5     | NOT ALFOSC                 | R    | 24.04±0.47 | 1.16±0.63   |      |                                         |
| 050724  | 5.6     | RTT 150                    | R    | >22.40     | <12.14      | 1.58 | <a href="#">Burenin et al. 2005</a>     |
|         | 58.7    | ESO/VLT FORS1              | R    | >24.40     | <1.62       |      | <a href="#">Malesani et al. (2007)</a>  |
|         | 82.8    | ESO/VLT FORS1              | R    | >24.80     | <1.12       |      |                                         |
|         | 779.2   | ESO/VLT FORS1              | R    | >25.70     | <0.49       |      |                                         |
|         | 83.2    | ESO/VLT FORS1              | V    | >25.45     | <1.04       |      |                                         |
| 070714B | 24.7    | WHT                        | R    | 23.50±0.30 | 1.61±0.51   | 0.38 | GCN#6630                                |
|         | 105.5   | Keck I LRIS                | R    | 25.50±0.30 | 0.26±0.081  |      | GCN#6652                                |
|         | 24      | TNG NICS                   | K    | 21.00±0.30 | 2.75±0.87   |      | GCN#6635                                |
| 061006  | 3824.2  | VLT FORS1                  | I    | 23.05±0.12 | 2.20±0.26   | 0.87 | <a href="#">D’Avanzo et al. (2009)</a>  |
|         | 3214.9  | VLT ISAAC                  | K    | >21.20     | <2.40       |      |                                         |
|         | 3322.3  | VLT FORS2                  | B    | 25.92±0.12 | 0.49±0.06   |      |                                         |
|         | 3705    | VLT ISAAC                  | J    | 22.00±0.20 | 3.14±0.63   |      |                                         |
|         | 3823.8  | VLT FORS1                  | V    | 24.56±0.07 | 1.24±0.08   |      |                                         |
| 061201  | 393.2   | VLT FORS2                  | I    | > 24.80    | <0.33       | 0.20 | <a href="#">Stratta et al. (2007)</a>   |
|         | 321     | VLT FORS2                  | R    | > 24.90    | <0.39       |      |                                         |
|         | 4119.1  | VLT FORS2                  | R    | > 25.90    | <0.16       |      |                                         |
|         | 1.85    | Swift/UVOT                 | uvv  | > 21.23    | <14.15      |      |                                         |
|         | 0.96    | Swift/UVOT                 | uvb  | > 21.14    | <18.05      |      |                                         |
|         | 0.91    | Swift/UVOT                 | uvu  | 20.86±0.54 | 9.15±5.89   |      |                                         |
|         | 1       | Swift/UVOT                 | uvw2 | 19.94±0.41 | 10.47±4.80  |      |                                         |
|         | 2.4     | Swift/UVOT                 | uvw1 | 20.75±0.36 | 6.30±2.48   |      |                                         |
|         | 2.95    | Swift/UVOT                 | uvm2 | 21.44±0.54 | 2.98±1.92   |      |                                         |
|         | 12.7    | Swift/UVOT                 | uvw1 | 22.72±0.47 | 1.03±0.56   |      |                                         |
|         | 37.1    | Swift/UVOT                 | uvw1 | >22.97     | <0.82       |      |                                         |
| 061210  | 0.225   | MDM 1.3-m                  | I    | >18.50     | <102.8      | 0.09 | GCN#5906                                |
|         | 0.0467  | 2-m Faulkes N              | R    | >17.00     | <526.8      |      | GCN#5920                                |
|         | 68.7072 | MDM 1.3-m                  | R    | 20.90±0.20 | 4.51±2.93   |      | GCN#5925                                |
| 050509B | 0.37175 | 1.3m PAIRITEL              | J    | >19.30     | <71.79      | 0.05 | <a href="#">Bloom et al. (2006)</a>     |
|         | 0.37175 | 1.3m PAIRITEL              | H    | >19.50     | <59.41      |      |                                         |
|         | 0.37175 | 1.3m PAIRITEL              | Ks   | >18.95     | <98.36      |      |                                         |
|         | 0.55656 | 3.5m WIYN OPTIC CCD        | i    | >20.95     | <15.97      |      |                                         |
|         | 0.63008 | 3.5m WIYN OPTIC CCD        | i    | >22.05     | <5.80       |      |                                         |
|         | 2.35342 | 3.5m WIYN OPTIC CCD        | r    | >23.84     | <1.13       |      |                                         |
|         | 2.53008 | 3.5m WIYN OPTIC CCD        | r    | >23.85     | <1.12       |      |                                         |
|         | 2.70747 | 3.5m WIYN OPTIC CCD        | r    | >24.11     | <0.88       |      |                                         |
|         | 50.0906 | Keck I LRIS-B              | R    | >24.60     | <0.56       |      |                                         |
|         | 50.0906 | Keck I LRIS-B              | g    | >25.50     | <0.25       |      |                                         |
|         | 192.133 | Keck II ESI                | R    | >25.10     | <0.35       |      |                                         |
|         | 0.00828 | ROTSE-IIIb                 | R    | >17.21     | <502.9      |      | GCN#3382                                |
|         | 0.01828 | ROTSE-IIIb                 | R    | >18.59     | <141.1      |      |                                         |
|         | 0.06947 | ROTSE-IIIb                 | R    | >18.68     | <129.9      |      |                                         |
|         | 0.20753 | ROTSE-IIIb                 | R    | >19.42     | <65.69      |      |                                         |
|         | 0.00878 | RAPTOR-S                   | R    | >18.92     | <104.1      |      | GCN#3414                                |
|         | 0.02128 | RAPTOR-S                   | R    | >20.12     | <34.48      |      |                                         |
|         | 0.10667 | RAPTOR-S                   | R    | >20.92     | <16.50      |      |                                         |

Continued on next page

Table 2 – continued from previous page

|        |         |                      |       |            |                               |      |                                             |
|--------|---------|----------------------|-------|------------|-------------------------------|------|---------------------------------------------|
|        | 0.34528 | RAPTOR-S             | R     | >21.82     | <7.20                         |      |                                             |
|        | 0.72833 | RAPTOR-S             | R     | >21.92     | <6.57                         |      |                                             |
|        | 1.12111 | RAPTOR-S             | R     | >21.72     | <7.90                         |      |                                             |
|        | 0.63692 | 1.2m Mercator        | R     | >21.12     | <13.73                        |      | GCN#3384                                    |
|        | 0.17581 | 0.3m NMS             | I     | >19.04     | <92.06                        |      | GCN#3393                                    |
|        | 0.31108 | 0.3m NMS             | I     | >19.54     | <58.09                        |      |                                             |
|        | 0.23903 | Swift UVOT           | uvv   | >18.96     | <101.5                        |      | GCN#3397                                    |
|        | 0.23583 | Swift UVOT           | uvb   | >20.14     | <34.75                        |      |                                             |
|        | 1.08667 | Swift UVOT           | uvu   | >19.40     | <69.38                        |      |                                             |
|        | 11.5    | 1.0m ARIES           | R     | >22.12     | <5.46                         |      | GCN#3396                                    |
|        | 26.025  | Keck-I LRIS          | R     | >25.70     | <0.20                         |      | GCN#3409                                    |
|        | 44.775  | ESO/VLT FORS         | R     | >26.60     | <0.07                         |      | <a href="#">Hjorth et al. (2005)</a>        |
|        | 94.455  | ESO/VLT FORS         | V     | >27.50     | <0.04                         |      |                                             |
|        | 190.57  | ESO/VLT FORS         | V     | >25.00     | <0.39                         |      |                                             |
|        | 285.37  | ESO/VLT FORS         | V     | >24.20     | <0.81                         |      |                                             |
|        | 548.295 | ESO/VLT FORS         | R     | >26.70     | <0.07                         |      |                                             |
|        | 549.015 | ESO/VLT FORS         | V     | >27.50     | <0.04                         |      |                                             |
|        | 0.66133 | 1.2m Mercator MEROPE | R     | >21.00     | <12.87                        |      | <a href="#">Castro-Tirado et al. (2005)</a> |
|        | 19.6613 | 1.2m Mercator MEROPE | R     | >22.10     | <4.67                         |      |                                             |
|        | 63.9947 | 6m BTA SCORPIO       | R     | >26.00     | <0.13                         |      |                                             |
|        | 234.995 | 1.5m OSN CCD         | I     | >21.90     | <4.41                         |      |                                             |
|        | 449.945 | 2.2m CAHA BUSCA      | R     | >23.90     | <0.89                         |      |                                             |
|        | 17.3447 | 3.5m CAHA OMEGA2000  | H     | >20.20     | <8.51                         |      |                                             |
|        | 19.3613 | 3.5m CAHA OMEGA2000  | K     | >18.80     | <20.17                        |      |                                             |
|        | 20.078  | 3.5m CAHA OMEGA2000  | J     | >21.20     | <5.30                         |      |                                             |
|        | 22.478  | 3.5m CAHA OMEGA2000  | H     | >20.50     | <6.45                         |      |                                             |
|        | 41.828  | 3.5m CAHA OMEGA2000  | J     | >20.30     | <12.14                        |      |                                             |
|        | 89.9113 | 3.5m CAHA OMEGA2000  | H     | >20.30     | <7.76                         |      |                                             |
|        | 162.478 | 3.5m CAHA OMEGA2000  | J     | >21.70     | <3.34                         |      |                                             |
|        | 210.995 | 3.5m CAHA OMEGA2000  | J     | >22.20     | <2.11                         |      |                                             |
|        | 9.94486 | Swift/UVOT           | uvv   | >21.10     | <13.89                        |      | GCN#3412                                    |
|        | 9.72417 | Swift/UVOT           | uvb   | >21.80     | <8.19                         |      |                                             |
|        | 10.6799 | Swift/UVOT           | uvu   | >21.80     | <3.11                         |      |                                             |
|        | 10.65   | Swift/UVOT           | uvw1  | >22.30     | <1.14                         |      |                                             |
|        | 10.5218 | Swift/UVOT           | uvm2  | >22.20     | <0.99                         |      |                                             |
|        | 9.8525  | Swift/UVOT           | uvw2  | >22.70     | <0.59                         |      |                                             |
| 050709 | 104.923 | VLT FORS1            | I     | >24.10     | <0.58                         | 0.03 | <a href="#">Watson et al. (2006)</a>        |
|        | 135.49  | Subaru               | K     | 22.10±0.70 | 0.96±0.87                     |      |                                             |
|        | 177.149 | 1.54m Danish DFOSC   | R     | >24.10     | <0.73                         |      |                                             |
|        | 418.507 | 1.54m Danish DFOSC   | R     | >24.00     | <0.80                         |      |                                             |
|        | 466.886 | 1.54m Danish DFOSC   | R     | >23.80     | <0.96                         |      |                                             |
|        | 484.006 | VLT FORS2            | V     | >25.20     | <0.31                         |      |                                             |
|        | 484.289 | VLT FORS2            | R     | >25.00     | <0.32                         |      |                                             |
|        | 485.556 | VLT FORS2            | I     | >23.50     | <1.00                         |      |                                             |
|        | 447.19  | HST ACS              | F814W | 27.81±0.27 | (28.38±8.01)×10 <sup>-3</sup> |      | <a href="#">Fox et al. (2005)</a>           |
|        | 29.76   | 40in Swope           | i     | >20.50     | <23.86                        |      |                                             |
|        | 27.5    | PROMPT-5             | R     | >21.00     | <12.68                        |      | GCN#3569                                    |
|        | 28.4    | 0.3m Bronberg        | R     | >19.50     | <50.46                        |      | GCN#3571                                    |
|        | 44.385  | Swift/UVOT           | uvv   | >21.64     | <8.28                         |      | GCN#3577                                    |
|        | 29.6    | PROMPT-5             | R     | >21.60     | <7.29                         |      | GCN#3702                                    |
|        | 201.05  | PROMPT-5             | R     | >21.60     | <7.29                         |      |                                             |
|        | 159.441 | Gemini-N             | R     | >25.40     | <0.22                         |      | <a href="#">Jin et al. (2016)</a>           |
|        | 251.656 | VLT FORS1            | V     | >24.50     | <0.60                         |      |                                             |
|        | 251.506 | VLT FORS1            | R     | >24.60     | <0.46                         |      |                                             |
|        | 58.9231 | VLT FORS2            | I     | 24.10±0.20 | 0.58±0.12                     |      |                                             |
|        | 200.023 | VLT FORS1            | I     | >24.80     | <0.31                         |      |                                             |
| 071227 | 4.6     | REM                  | R     | >17.00     | <506.5                        | 0.03 | GCN#7149                                    |
|        | 4.6     | REM                  | H     | >15.50     | <643.7                        |      |                                             |

Continued on next page

Table 2 – continued from previous page

|         |         |                               |         |        |        |      |                                                  |
|---------|---------|-------------------------------|---------|--------|--------|------|--------------------------------------------------|
|         | 0.1852  | Swift/UVOT                    | uvv     | >20.46 | <24.66 |      | GCN#7150                                         |
|         | 0.5546  | Swift/UVOT                    | uvb     | >21.01 | <16.61 |      |                                                  |
|         | 0.5347  | Swift/UVOT                    | uvu     | >20.33 | <11.78 |      |                                                  |
|         | 0.5152  | Swift/UVOT                    | uvw1    | >20.17 | <7.84  |      |                                                  |
|         | 0.7093  | Swift/UVOT                    | uvm2    | >21.00 | <2.85  |      |                                                  |
|         | 0.5862  | Swift/UVOT                    | uvw2    | >20.65 | <3.73  |      |                                                  |
|         | 7.7     | Magellan/Baade IMACS          | R       | >22.30 | <3.84  |      | GCN#7151                                         |
|         | 4.1575  | ESO/MPG GROND                 | r       | >20.60 | <21.97 |      | <a href="#">Nicuesa Guelbenzu et al. (2012b)</a> |
|         | 4.1575  | ESO/MPG GROND                 | i       | >20.00 | <37.94 |      |                                                  |
|         | 4.1575  | ESO/MPG GROND                 | z       | >20.40 | <26.09 |      |                                                  |
|         | 4.1575  | ESO/MPG GROND                 | J       | >20.00 | <37.52 |      |                                                  |
|         | 4.1575  | ESO/MPG GROND                 | H       | >19.80 | <44.95 |      |                                                  |
|         | 4.1575  | ESO/MPG GROND                 | Ks      | >19.40 | <64.87 |      |                                                  |
|         | 29      | ESO/MPG GROND                 | g       | >25.50 | <0.24  |      |                                                  |
|         | 29      | ESO/MPG GROND                 | r       | >25.00 | <0.38  |      |                                                  |
|         | 29      | ESO/MPG GROND                 | i       | >24.20 | <0.79  |      |                                                  |
|         | 29      | ESO/MPG GROND                 | z       | >24.40 | <0.66  |      |                                                  |
|         | 29      | ESO/MPG GROND                 | J       | >21.50 | <9.42  |      |                                                  |
|         | 29      | ESO/MPG GROND                 | H       | >20.50 | <23.59 |      |                                                  |
| 060502B | 1       | 0.8m Xinglong Obs             | R       | >20.60 | <19.44 | 0.11 | GCN#5057                                         |
|         | 2.6424  | Tautenburg 1.34m Schmidt Tel. | R       | >20.20 | <28.1  |      | GCN#5062                                         |
|         | 0.0886  | 0.3m AGU Japan                | R       | >16.00 | <1345  |      | GCN#5065                                         |
|         | 0.3942  | Swift UVOT                    | uvv     | >20.29 | <31.05 |      | GCN#5069                                         |
|         | 1.1167  | Swift UVOT                    | uvb     | >20.62 | <26.22 |      |                                                  |
|         | 1.4182  | Swift UVOT                    | uvu     | >21.04 | <6.86  |      |                                                  |
|         | 1.3755  | Swift UVOT                    | uvw1    | >21.29 | <3.25  |      |                                                  |
|         | 1.2781  | Swift UVOT                    | uvm2    | >21.31 | <2.66  |      |                                                  |
|         | 1.3497  | Swift UVOT                    | uvw2    | >21.29 | <2.48  |      |                                                  |
|         | 0.1977  | Swift UVOT                    | uvwhite | >20.49 | <13.84 |      |                                                  |
|         | 0.0886  | Moscow Union Optic MAS-TER    | R       | >16.12 | <1204  |      | GCN#5073                                         |
|         | 0.215   | Moscow Union Optic MAS-TER    | R       | >16.26 | <1058  |      |                                                  |
|         | 0.34222 | Moscow Union Optic MAS-TER    | R       | >16.00 | <1345  |      |                                                  |
|         | 0.4675  | Moscow Union Optic MAS-TER    | R       | >16.00 | <1345  |      |                                                  |
|         | 0.5922  | Moscow Union Optic MAS-TER    | R       | >16.30 | <1020  |      |                                                  |
|         | 5.68    | 152 Cassini tel Loiano BFOSC  | R       | >20.60 | <19.44 |      | GCN#5074                                         |
| 070724A | 40.8    | Gemini Noth GMOS              | r       | >24.70 | <0.54  |      | GCN#5077                                         |
|         | 2.3064  | UKIRT UFTI                    | K       | >18.05 | <40.18 | 0.04 | <a href="#">Kocevski et al. (2010)</a>           |
|         | 2.5368  | UKIRT UFTI                    | J       | >19.62 | <22.61 |      |                                                  |
|         | 3.048   | UKIRT UFTI                    | H       | >18.88 | <28.63 |      |                                                  |
|         | 3.1584  | UKIRT UFTI                    | K       | >18.35 | <30.48 |      |                                                  |
|         | 17.4096 | NOT StanCam                   | i       | >23.47 | <1.55  |      |                                                  |
|         | 17.7216 | NOT StanCam                   | R       | >23.72 | <1.04  |      |                                                  |
|         | 18.336  | NOT StanCam                   | B       | >21.95 | <6.87  |      |                                                  |
|         | 21.3504 | 1.3m CTIO ANDICAM             | J       | >20.67 | <8.60  |      |                                                  |
|         | 21.3528 | 1.3m CTIO ANDICAM             | I       | >21.79 | <4.84  |      |                                                  |
|         | 22.2504 | VLT FORS2                     | i       | >24.74 | <0.48  |      |                                                  |
|         | 27.048  | UKIRT UFTI                    | K       | >17.47 | <68.54 |      |                                                  |
|         | 68.3712 | 1.3m CTIO ANDICAM             | J       | >20.80 | <7.63  |      |                                                  |
|         | 68.3712 | 1.3m CTIO ANDICAM             | I       | >21.95 | <4.18  |      |                                                  |
|         | 117.979 | 1.3m CTIO ANDICAM             | J       | >19.16 | <34.54 |      |                                                  |
|         | 117.979 | 1.3m CTIO ANDICAM             | I       | >21.85 | <4.58  |      |                                                  |

Continued on next page

Table 2 – continued from previous page

|         |         |                   |         |            |             |                                          |
|---------|---------|-------------------|---------|------------|-------------|------------------------------------------|
|         | 166.164 | 1.3m CTIO ANDICAM | J       | >19.46     | <26.20      |                                          |
|         | 166.164 | 1.3m CTIO ANDICAM | I       | >21.90     | <4.38       |                                          |
|         | 237.737 | 1.3m CTIO ANDICAM | J       | >19.93     | <17.00      |                                          |
|         | 237.737 | 1.3m CTIO ANDICAM | I       | >20.70     | <13.22      |                                          |
|         | 333.734 | 1.3m CTIO ANDICAM | J       | >19.99     | <16.08      |                                          |
|         | 333.619 | 1.3m CTIO ANDICAM | I       | >21.71     | <5.21       |                                          |
|         | 406.534 | 1.3m CTIO ANDICAM | I       | >21.83     | <4.67       |                                          |
|         | 434.772 | Keck I LRIS       | R       | >25.10     | <0.29       |                                          |
|         | 434.772 | Keck I LRIS       | g       | >23.32     | <1.82       |                                          |
|         | 434.93  | Keck I LRIS       | R       | >23.39     | <1.41       |                                          |
|         | 434.969 | Keck I LRIS       | R       | >23.26     | <1.59       |                                          |
|         | 435.017 | Keck I LRIS       | R       | >25.39     | <0.22       |                                          |
|         | 435.137 | Keck I LRIS       | g       | >25.00     | <0.39       |                                          |
|         | 435.218 | Keck I LRIS       | R       | >25.37     | <0.23       |                                          |
|         | 435.221 | Keck I LRIS       | g       | >25.50     | <0.24       |                                          |
|         | 435.413 | Keck I LRIS       | g       | >25.70     | <0.20       |                                          |
|         | 435.415 | Keck I LRIS       | R       | >25.44     | <0.21       |                                          |
|         | 435.614 | Keck I LRIS       | R       | >25.44     | <0.21       |                                          |
|         | 435.614 | Keck I LRIS       | g       | >25.80     | <0.18       |                                          |
|         | 435.398 | Keck I LRIS       | R       | >27.40     | <0.04       |                                          |
|         | 435.504 | Keck I LRIS       | g       | >26.25     | <0.12       |                                          |
|         | 502.198 | 1.3m CTIO ANDICAM | J       | >19.77     | <19.70      |                                          |
|         | 502.2   | 1.3m CTIO ANDICAM | I       | >21.33     | <7.40       |                                          |
|         | 544.699 | NOT StanCam       | R       | >24.80     | <0.38       |                                          |
|         | 573.509 | 1.3m CTIO ANDICAM | J       | >20.00     | <15.94      |                                          |
|         | 573.509 | 1.3m CTIO ANDICAM | I       | >21.63     | <5.61       |                                          |
|         | 622.378 | 1.3m CTIO ANDICAM | J       | >20.02     | <15.64      |                                          |
|         | 622.378 | 1.3m CTIO ANDICAM | I       | >21.67     | <5.41       |                                          |
|         | 668.623 | 1.3m CTIO ANDICAM | J       | >20.21     | <13.13      |                                          |
|         | 668.623 | 1.3m CTIO ANDICAM | I       | >22.11     | <3.61       |                                          |
|         | 0.035   | Swift UVOT        | uvwhite | >20.40     | <13.10      | GCN#6660                                 |
|         | 0.10597 | Swift UVOT        | uvv     | >19.50     | <59.78      |                                          |
|         | 0.77875 | Swift UVOT        | uvwhite | >21.10     | <6.88       |                                          |
|         | 0.85042 | Swift UVOT        | uvv     | >20.00     | <37.72      |                                          |
|         | 0.83153 | Swift UVOT        | uvb     | >20.30     | <32.00      |                                          |
|         | 0.985   | Swift UVOT        | uvu     | >20.00     | <16.00      |                                          |
|         | 0.96722 | Swift UVOT        | uvw1    | >20.40     | <6.36       |                                          |
|         | 0.93514 | Swift UVOT        | uvm2    | >20.40     | <4.96       |                                          |
|         | 0.89278 | Swift UVOT        | uvw2    | >20.70     | <3.58       |                                          |
|         | 0.32    | P60               | i       | >21.50     | <9.54       | GCN#6664                                 |
|         | 0.371   | ESO/MPG GROND     | g       | –          | –           | –<br>Nicuesa Guelbenzu et al.<br>(2012a) |
| 100816A | 0.371   | ROTSE-IIIc        | R       | >16.60     | <837.2      | 0.23 GCN#11103                           |
|         | 0.426   | ROTSE-IIIc        | R       | >18.50     | <145.5      |                                          |
|         | 2.8     | TNG DOLORES       | R       | 20.50±0.30 | 23.06±7.34  | GCN#11104                                |
|         | 0.375   | MASTER            | R       | >17.20     | <481.8      | GCN#11105                                |
|         | 0.407   | TAROT             | R       | 19.20±0.30 | 76.35±24.30 | GCN#11106                                |
|         | 8.03    | 2.1m/McDonald     | Obs. i  | 21.31±0.10 | 12.73±1.23  | GCN#11108                                |
|         |         | CQUEAN            |         |            |             |                                          |
|         | 11      | GEMINI-N GMOS     | R       | 22.40±0.30 | 4.01±1.28   | GCN#11109                                |
|         | 0.55    | Calar Alto        | I       | 19.90±0.30 | 30.07±9.57  | GCN#11112                                |
|         | 0.1655  | Swift UVOT        | uvwhite | 18.90±0.19 | 73.07±13.97 | GCN#11115                                |
|         | 1.3162  | Swift UVOT        | uvv     | 21.56±0.94 | 10.71±14.74 |                                          |
|         | 1.5405  | Swift UVOT        | uvb     | 21.07±0.35 | 19.90±7.57  |                                          |
|         | 1.3069  | Swift UVOT        | uvu     | 20.39±0.35 | 14.66±5.58  |                                          |
|         | 1.4317  | Swift UVOT        | uvw1    | 20.98±0.44 | 5.37±2.68   |                                          |
|         | 3.3429  | Swift UVOT        | uvm2    | >21.42     | <3.26       |                                          |
|         | 2.8944  | Swift UVOT        | uvw2    | >22.19     | <1.40       |                                          |
|         | 24.3    | NOT ALFOSC        | R       | 23.00±0.10 | 2.31±0.22   | GCN#11120                                |

Continued on next page

Table 2 – continued from previous page

|         |         |                   |    |            |            |       |                                  |
|---------|---------|-------------------|----|------------|------------|-------|----------------------------------|
|         | 13.4    | MITSUME           | V  | >21.00     | <18.10     |       | GCN#11126                        |
|         | 13.4    | MITSUME           | Rc | >20.50     | <22.92     |       |                                  |
|         | 13.4    | MITSUME           | I  | >19.90     | <30.07     |       |                                  |
|         | 48      | GTC               | r  | 25.00±0.20 | 0.44±0.09  |       | Pérez-Ramírez et al. (2013)      |
|         | 96      | GTC               | r  | 25.20±0.20 | 0.37±0.075 |       |                                  |
| 140903A | 14.4    | Gemini North GMOS | i  | 21.33±0.05 | 11.51±0.54 | 0.088 | Troja et al. (2016)              |
|         | 39.12   | Gemini North GMOS | i  | 22.99±0.13 | 2.49±0.32  |       |                                  |
|         | 12.72   | DCT LMI           | r  | 21.63±0.06 | 8.87±0.50  |       |                                  |
|         | 37.2    | DCT LMI           | r  | > 21.2     | <13.18     |       |                                  |
|         | 60      | DCT LMI           | r  | > 22.3     | <4.79      |       |                                  |
|         | 107.76  | DCT LMI           | r  | > 22.9     | <2.75      |       |                                  |
| 090510  | 6.42417 | ESO/MPG GROND     | g  | 22.88±0.56 | 2.79±1.89  | 0.06  | Nicuesa Guelbenzu et al. (2012b) |
|         | 6.56639 | ESO/MPG GROND     | g  | 22.9 ±0.36 | 2.74±1.08  |       |                                  |
|         | 6.94    | ESO/MPG GROND     | g  | 22.88±0.33 | 2.79±0.99  |       |                                  |
|         | 7.19139 | ESO/MPG GROND     | g  | 23.07±0.29 | 2.35±0.72  |       |                                  |
|         | 7.31528 | ESO/MPG GROND     | g  | 23.45±0.43 | 1.65±0.80  |       |                                  |
|         | 7.43889 | ESO/MPG GROND     | g  | 23.86±0.5  | 1.13±0.66  |       |                                  |
|         | 7.565   | ESO/MPG GROND     | g  | 23.54±0.37 | 1.52±0.62  |       |                                  |
|         | 7.68861 | ESO/MPG GROND     | g  | 23.41±0.27 | 1.72±0.48  |       |                                  |
|         | 7.8125  | ESO/MPG GROND     | g  | 23.61±0.33 | 1.43±0.51  |       |                                  |
|         | 8.06222 | ESO/MPG GROND     | g  | 23.52±0.35 | 1.55 ±0.59 |       |                                  |
|         | 8.1875  | ESO/MPG GROND     | g  | 23.43±0.31 | 1.68±0.56  |       |                                  |
|         | 8.6875  | ESO/MPG GROND     | g  | 23.7 ±0.32 | 1.31±0.45  |       |                                  |
|         | 8.8125  | ESO/MPG GROND     | g  | 23.77±0.34 | 1.23±0.45  |       |                                  |
|         | 8.93611 | ESO/MPG GROND     | g  | 23.91±0.31 | 1.08±0.36  |       |                                  |
|         | 9.06333 | ESO/MPG GROND     | g  | 23.75±0.33 | 1.25±0.45  |       |                                  |
|         | 9.18806 | ESO/MPG GROND     | g  | 23.5 ±0.21 | 1.58±0.34  |       |                                  |
|         | 9.54694 | ESO/MPG GROND     | g  | 24.46±0.57 | 0.65±0.45  |       |                                  |
|         | 9.67083 | ESO/MPG GROND     | g  | 24.19±0.31 | 0.84±0.28  |       |                                  |
|         | 9.79722 | ESO/MPG GROND     | g  | 23.9 ±0.31 | 1.09±0.36  |       |                                  |
|         | 9.92083 | ESO/MPG GROND     | g  | 24.21±0.43 | 0.82±0.40  |       |                                  |
|         | 6.19417 | ESO/MPG GROND     | r  | 22.01±0.38 | 6.12±2.56  |       |                                  |
|         | 6.25083 | ESO/MPG GROND     | r  | 22.09±0.38 | 5.68±2.38  |       |                                  |
|         | 6.3175  | ESO/MPG GROND     | r  | 22.29±0.33 | 4.73±1.68  |       |                                  |
|         | 6.36972 | ESO/MPG GROND     | r  | 22.89±0.57 | 2.72 ±1.88 |       |                                  |
|         | 6.42417 | ESO/MPG GROND     | r  | 22.73±0.51 | 3.15±1.89  |       |                                  |
|         | 6.47583 | ESO/MPG GROND     | r  | 22.91±0.53 | 2.67 ±1.68 |       |                                  |
|         | 6.6925  | ESO/MPG GROND     | r  | 23.03±0.29 | 2.39±0.73  |       |                                  |
|         | 6.81667 | ESO/MPG GROND     | r  | 22.49±0.2  | 3.93±0.80  |       |                                  |
|         | 6.94    | ESO/MPG GROND     | r  | 22.86±0.31 | 2.80±0.92  |       |                                  |
|         | 7.0675  | ESO/MPG GROND     | r  | 22.62±0.23 | 3.49±0.82  |       |                                  |
|         | 7.19139 | ESO/MPG GROND     | r  | 22.77±0.24 | 3.04±0.75  |       |                                  |
|         | 7.31528 | ESO/MPG GROND     | r  | 23.09±0.32 | 2.26±0.78  |       |                                  |
|         | 7.43889 | ESO/MPG GROND     | r  | 22.71±0.24 | 3.21 ±0.79 |       |                                  |
|         | 7.565   | ESO/MPG GROND     | r  | 23.05±0.25 | 2.35±0.61  |       |                                  |
|         | 7.68861 | ESO/MPG GROND     | r  | 23.26±0.21 | 1.93±0.41  |       |                                  |
|         | 7.8125  | ESO/MPG GROND     | r  | 23.23±0.25 | 1.99±0.51  |       |                                  |
|         | 7.93583 | ESO/MPG GROND     | r  | 23.07±0.24 | 2.30±0.57  |       |                                  |
|         | 8.06222 | ESO/MPG GROND     | r  | 23.3 ±0.31 | 1.86±0.62  |       |                                  |
|         | 8.1875  | ESO/MPG GROND     | r  | 23.17±0.25 | 2.10±0.54  |       |                                  |
|         | 8.31167 | ESO/MPG GROND     | r  | 23.19±0.23 | 2.06±0.49  |       |                                  |
|         | 8.4375  | ESO/MPG GROND     | r  | 23.11±0.21 | 2.22±0.47  |       |                                  |
|         | 8.56417 | ESO/MPG GROND     | r  | 23.01±0.2  | 2.44±0.49  |       |                                  |
|         | 8.6875  | ESO/MPG GROND     | r  | 23.19±0.23 | 2.06±0.49  |       |                                  |
|         | 8.8125  | ESO/MPG GROND     | r  | 23.25±0.23 | 1.95±0.46  |       |                                  |
|         | 8.93611 | ESO/MPG GROND     | r  | 23.48±0.29 | 1.58 ±0.48 |       |                                  |
|         | 9.06333 | ESO/MPG GROND     | r  | 23.38±0.25 | 1.73±0.45  |       |                                  |

Continued on next page

Table 2 – continued from previous page

|         |               |                     |            |            |       |
|---------|---------------|---------------------|------------|------------|-------|
| 9.18806 | ESO/MPG GROND | r                   | 23.67±0.3  | 1.33±0.42  |       |
| 9.31222 | ESO/MPG GROND | r                   | 23.52±0.27 | 1.52±0.43  |       |
| 9.54694 | ESO/MPG GROND | r                   | 23.51±0.26 | 1.54±0.42  |       |
| 9.67083 | ESO/MPG GROND | r                   | 24.07±0.46 | 0.92±0.48  |       |
| 9.79722 | ESO/MPG GROND | r                   | 23.74±0.32 | 1.24±0.43  |       |
| 6.28028 | ESO/MPG GROND | i                   | 21.85±0.4  | 7.01±3.12  |       |
| 6.36972 | ESO/MPG GROND | i                   | 22.16±0.38 | 5.27±2.21  |       |
| 6.42417 | ESO/MPG GROND | i                   | 21.86±0.35 | 6.95±2.64  |       |
| 6.47583 | ESO/MPG GROND | i                   | 21.81±0.34 | 7.27±2.68  |       |
| 6.56639 | ESO/MPG GROND | i                   | 22.35±0.31 | 4.42±1.46  |       |
| 6.6925  | ESO/MPG GROND | i                   | 22.18±0.2  | 5.17±1.05  |       |
| 6.81667 | ESO/MPG GROND | i                   | 22.79±0.45 | 2.95 ±1.52 |       |
| 6.94    | ESO/MPG GROND | i                   | 22.53±0.33 | 3.75±1.33  |       |
| 7.0675  | ESO/MPG GROND | i                   | 22.86±0.39 | 2.77±1.20  |       |
| 7.19139 | ESO/MPG GROND | i                   | 22.98±0.41 | 2.48±1.14  |       |
| 7.43889 | ESO/MPG GROND | i                   | 23.14±0.27 | 2.14±0.60  |       |
| 7.565   | ESO/MPG GROND | i                   | 22.5 ±0.2  | 3.85±0.78  |       |
| 7.68861 | ESO/MPG GROND | i                   | 22.58±0.18 | 3.57±0.65  |       |
| 7.8125  | ESO/MPG GROND | i                   | 22.81±0.26 | 2.90±0.78  |       |
| 7.93583 | ESO/MPG GROND | i                   | 22.76±0.27 | 3.03±0.86  |       |
| 8.06222 | ESO/MPG GROND | i                   | 22.84±0.26 | 2.82±0.76  |       |
| 8.1875  | ESO/MPG GROND | i                   | 22.97±0.29 | 2.50±0.77  |       |
| 8.31167 | ESO/MPG GROND | i                   | 22.99±0.33 | 2.45±0.87  |       |
| 8.4375  | ESO/MPG GROND | i                   | 23.03±0.29 | 2.37±0.72  |       |
| 8.56417 | ESO/MPG GROND | i                   | 22.91±0.3  | 2.64±0.84  |       |
| 8.6875  | ESO/MPG GROND | i                   | 23.23±0.22 | 1.97±0.44  |       |
| 8.8125  | ESO/MPG GROND | i                   | 23.08±0.2  | 2.26±0.46  |       |
| 8.93611 | ESO/MPG GROND | i                   | 23.58±0.41 | 1.43±0.65  |       |
| 9.06333 | ESO/MPG GROND | i                   | 23.01±0.28 | 2.41±0.71  |       |
| 9.18806 | ESO/MPG GROND | i                   | 23.26±0.29 | 1.91±0.59  |       |
| 9.31222 | ESO/MPG GROND | i                   | 22.99±0.15 | 2.45±0.36  |       |
| 9.54694 | ESO/MPG GROND | i                   | 23.83±0.52 | 1.13±0.70  |       |
| 9.79722 | ESO/MPG GROND | i                   | 23.23±0.29 | 1.97±0.60  |       |
| 9.92083 | ESO/MPG GROND | i                   | 23.9 ±0.57 | 1.06±0.73  |       |
| 6.19417 | ESO/MPG GROND | i                   | 21.73±0.56 | 7.83 ±5.29 |       |
| 6.2225  | ESO/MPG GROND | i                   | 21.27±0.4  | 11.96±5.33 |       |
| 6.28028 | ESO/MPG GROND | i                   | 21.41±0.4  | 10.51±4.68 |       |
| 6.3175  | ESO/MPG GROND | i                   | 21.45±0.28 | 10.13±2.98 |       |
| 6.56639 | ESO/MPG GROND | i                   | 22.09±0.32 | 5.62 ±1.93 |       |
| 6.6925  | ESO/MPG GROND | i                   | 22.4 ±0.45 | 4.22±2.17  |       |
| 6.94    | ESO/MPG GROND | i                   | 22.5 ±0.36 | 3.85±1.52  |       |
| 7.19139 | ESO/MPG GROND | i                   | 22.95±0.45 | 2.55±1.31  |       |
| 7.31528 | ESO/MPG GROND | i                   | 21.95±0.23 | 6.39±1.51  |       |
| 7.565   | ESO/MPG GROND | i                   | 22.55±0.29 | 3.68±1.13  |       |
| 7.8125  | ESO/MPG GROND | i                   | 22.88±0.37 | 2.72±1.10  |       |
| 7.93583 | ESO/MPG GROND | i                   | 22.63±0.31 | 3.42±1.13  |       |
| 8.06222 | ESO/MPG GROND | i                   | 22.26±0.24 | 4.81±1.19  |       |
| 8.1875  | ESO/MPG GROND | i                   | 22.77±0.4  | 3.00±1.34  |       |
| 8.4375  | ESO/MPG GROND | i                   | 22.98±0.4  | 2.48±1.10  |       |
| 8.56417 | ESO/MPG GROND | i                   | 22.96±0.46 | 2.52±1.33  |       |
| 8.8125  | ESO/MPG GROND | i                   | 22.56±0.23 | 3.65±0.860 |       |
| 9.06333 | ESO/MPG GROND | i                   | 23.18±0.46 | 2.06±1.09  |       |
| 9.18806 | ESO/MPG GROND | i                   | 23.01±0.29 | 2.41±0.74  |       |
| 9.79722 | ESO/MPG GROND | i                   | 23.44±0.43 | 1.62±0.79  |       |
| 9.92083 | ESO/MPG GROND | i                   | 23.11±0.41 | 2.20±1.01  |       |
| 061217  | 2.8           | Magellan Clay LDSS3 | r          | >23.2      | <2.15 |

Berger et al. (2007)

Berger et al. (2007)

Table 3: Rest frame light-curves of AT2017gfo

| time<br>days | Luminosity<br>[erg/s/Hz] | M <sub>abs</sub><br>AB | filter | time<br>days | Luminosity<br>[erg/s/Hz] | M <sub>abs</sub><br>AB | filter |
|--------------|--------------------------|------------------------|--------|--------------|--------------------------|------------------------|--------|
| 0.50         | —                        | —                      | U      | 0.50         | 1.12308E+27              | −16.01                 | I      |
| 0.64         | 7.18098E+26              | −15.52                 | U      | 0.64         | 1.05270E+27              | −15.93                 | I      |
| 0.99         | 3.80807E+26              | −14.83                 | U      | 0.99         | 8.92441E+26              | −15.76                 | I      |
| 1.49         | 1.01852E+26              | −13.40                 | U      | 1.49         | 6.79025E+26              | −15.46                 | I      |
| 2.43         | 1.65102E+25              | −11.42                 | U      | 2.43         | 4.07835E+26              | −14.91                 | I      |
| 3.47         | 5.34701E+24              | −10.20                 | U      | 3.47         | 2.51014E+26              | −14.38                 | I      |
| 4.41         | 4.50884E+24              | −10.01                 | U      | 4.41         | 1.94470E+26              | −14.10                 | I      |
| 5.45         | 3.18208E+24              | −9.64                  | U      | 5.45         | 1.32060E+26              | −13.68                 | I      |
| 6.44         | 2.99461E+24              | −9.57                  | U      | 6.44         | 8.36330E+25              | −13.19                 | I      |
| 7.43         | 3.21350E+24              | −9.65                  | U      | 7.43         | 6.32492E+25              | −12.88                 | I      |
| 8.42         | 3.11434E+24              | −9.61                  | U      | 8.42         | 4.65145E+25              | −12.55                 | I      |
| 9.41         | 2.43233E+24              | −9.34                  | U      | 9.41         | 3.63476E+25              | −12.28                 | I      |
| 10.40        | 2.31444E+24              | −9.29                  | U      | 10.40        | 2.81474E+25              | −12.00                 | I      |
| 11.39        | 2.01956E+24              | −9.14                  | U      | 11.39        | 1.30292E+25              | −11.17                 | I      |
| 0.64         | 1.00179E+27              | −15.88                 | B      | 0.64         | 1.04545E+27              | −15.93                 | g      |
| 0.99         | 6.16056E+26              | −15.35                 | B      | 0.99         | 6.76941E+26              | −15.46                 | g      |
| 1.49         | 2.85252E+26              | −14.52                 | B      | 1.49         | 3.49269E+26              | −14.74                 | g      |
| 2.43         | 6.15227E+25              | −12.85                 | B      | 2.43         | 8.75915E+25              | −13.24                 | g      |
| 3.47         | 2.30480E+25              | −11.79                 | B      | 3.47         | 3.35735E+25              | −12.19                 | g      |
| 4.41         | 1.38806E+25              | −11.24                 | B      | 4.41         | 2.15770E+25              | −11.71                 | g      |
| 5.45         | 1.05682E+25              | −10.94                 | B      | 5.45         | 1.50837E+25              | −11.33                 | g      |
| 6.44         | 7.80296E+24              | −10.61                 | B      | 6.44         | 9.69888E+24              | −10.85                 | g      |
| 7.43         | 7.71662E+24              | −10.60                 | B      | 7.43         | 9.30613E+24              | −10.80                 | g      |
| 8.42         | 7.92575E+24              | −10.63                 | B      | 8.42         | 1.06830E+25              | −10.95                 | g      |
| 9.41         | 7.95381E+24              | −10.63                 | B      | 9.41         | 9.27390E+24              | −10.80                 | g      |
| 10.40        | 7.80186E+24              | −10.61                 | B      | 10.40        | 9.19524E+24              | −10.79                 | g      |
| 11.39        | 6.03662E+24              | −10.33                 | B      | 11.39        | 6.29801E+24              | −10.38                 | g      |
| 0.50         | 1.15013E+27              | −16.03                 | V      | 0.50         | 1.29382E+27              | −16.16                 | r      |
| 0.64         | 1.01439E+27              | −15.89                 | V      | 0.64         | 1.14902E+27              | −16.03                 | r      |
| 0.99         | 7.35529E+26              | −15.55                 | V      | 0.99         | 8.50274E+26              | −15.70                 | r      |
| 1.49         | 5.00401E+26              | −15.13                 | V      | 1.49         | 6.21757E+26              | −15.36                 | r      |
| 2.43         | 1.62837E+26              | −13.91                 | V      | 2.43         | 2.43402E+26              | −14.35                 | r      |
| 3.47         | 6.75307E+25              | −12.95                 | V      | 3.47         | 1.17989E+26              | −13.56                 | r      |
| 4.41         | 4.58176E+25              | −12.53                 | V      | 4.41         | 6.90316E+25              | −12.98                 | r      |
| 5.45         | 2.66279E+25              | −11.94                 | V      | 5.45         | 4.63674E+25              | −12.54                 | r      |
| 6.44         | 1.68206E+25              | −11.44                 | V      | 6.44         | 3.02903E+25              | −12.08                 | r      |
| 7.43         | 1.64037E+25              | −11.42                 | V      | 7.43         | 2.64714E+25              | −11.94                 | r      |
| 8.42         | 1.65927E+25              | −11.43                 | V      | 8.42         | 2.46373E+25              | −11.86                 | r      |
| 9.41         | 1.21946E+25              | −11.09                 | V      | 9.41         | 2.04940E+25              | −11.66                 | r      |
| 10.40        | 1.26556E+25              | −11.13                 | V      | 10.40        | 1.89003E+25              | −11.57                 | r      |
| 11.39        | 8.12694E+24              | −10.65                 | V      | 11.39        | 9.51188E+24              | −10.82                 | r      |
| 0.50         | 1.33263E+27              | −16.19                 | R      | 0.50         | 1.27211E+27              | −16.14                 | i      |
| 0.64         | 1.18982E+27              | −16.07                 | R      | 0.64         | 1.16239E+27              | −16.04                 | i      |
| 0.99         | 8.94234E+26              | −15.76                 | R      | 0.99         | 9.27863E+26              | −15.80                 | i      |
| 1.49         | 6.50428E+26              | −15.41                 | R      | 1.49         | 6.69659E+26              | −15.44                 | i      |
| 2.43         | 2.83216E+26              | −14.51                 | R      | 2.43         | 3.82166E+26              | −14.83                 | i      |
| 3.47         | 1.52744E+26              | −13.84                 | R      | 3.47         | 2.30523E+26              | −14.29                 | i      |
| 4.41         | 9.37159E+25              | −13.31                 | R      | 4.41         | 1.63926E+26              | −13.92                 | i      |
| 5.45         | 5.98498E+25              | −12.82                 | R      | 5.45         | 1.05893E+26              | −13.44                 | i      |
| 6.44         | 3.82656E+25              | −12.34                 | R      | 6.44         | 6.66017E+25              | −12.94                 | i      |
| 7.43         | 3.22239E+25              | −12.15                 | R      | 7.43         | 5.15043E+25              | −12.66                 | i      |
| 8.42         | 2.78513E+25              | −11.99                 | R      | 8.42         | 3.81874E+25              | −12.33                 | i      |
| 9.41         | 2.04888E+25              | −11.66                 | R      | 9.41         | 3.11568E+25              | −12.11                 | i      |
| 10.40        | 2.03389E+25              | −11.65                 | R      | 10.40        | 2.54864E+25              | −11.89                 | i      |
| 11.39        | 1.01911E+25              | −10.90                 | R      | 11.39        | 1.24449E+25              | −11.12                 | i      |
| 0.50         | 1.12308E+27              | −16.01                 | I      | 0.50         | 9.67550E+26              | −15.84                 | z      |

Continued on next page

Table 3 – continued from previous page

|       |             |        |   |       |             |        |   |
|-------|-------------|--------|---|-------|-------------|--------|---|
| 0.64  | 1.05270E+27 | -15.93 | I | 0.64  | 9.42562E+26 | -15.81 | z |
| 0.99  | 8.92441E+26 | -15.76 | I | 0.99  | 8.75996E+26 | -15.74 | z |
| 1.49  | 6.79025E+26 | -15.46 | I | 1.49  | 7.50386E+26 | -15.57 | z |
| 2.43  | 4.07835E+26 | -14.91 | I | 2.43  | 4.70720E+26 | -15.06 | z |
| 3.47  | 2.51014E+26 | -14.38 | I | 3.47  | 2.87708E+26 | -14.53 | z |
| 4.41  | 1.94470E+26 | -14.10 | I | 4.41  | 2.37385E+26 | -14.32 | z |
| 5.45  | 1.32060E+26 | -13.68 | I | 5.45  | 1.67421E+26 | -13.94 | z |
| 6.44  | 8.36330E+25 | -13.19 | I | 6.44  | 1.12707E+26 | -13.51 | z |
| 7.43  | 6.32492E+25 | -12.88 | I | 7.43  | 8.48137E+25 | -13.20 | z |
| 8.42  | 4.65145E+25 | -12.55 | I | 8.42  | 6.04742E+25 | -12.83 | z |
| 9.41  | 3.63476E+25 | -12.28 | I | 9.41  | 4.47893E+25 | -12.51 | z |
| 10.40 | 2.81474E+25 | -12.00 | I | 10.40 | 3.57482E+25 | -12.26 | z |
| 11.39 | 1.30292E+25 | -11.17 | I | 11.39 | 1.81244E+25 | -11.52 | z |
| 0.50  | -           | -      | g | 0.50  | 9.32020E+26 | -15.80 | J |
| 0.64  | 1.04545E+27 | -15.93 | g | 0.64  | 9.36659E+26 | -15.81 | J |
| 0.99  | 6.76941E+26 | -15.46 | g | 0.99  | 9.39742E+26 | -15.81 | J |
| 1.49  | 3.49269E+26 | -14.74 | g | 1.49  | 7.41414E+26 | -15.55 | J |
| 2.43  | 8.75915E+25 | -13.24 | g | 2.43  | 6.91296E+26 | -15.48 | J |
| 3.47  | 3.35735E+25 | -12.19 | g | 3.47  | 5.14759E+26 | -15.16 | J |
| 4.41  | 2.15770E+25 | -11.71 | g | 4.41  | 4.18133E+26 | -14.93 | J |
| 5.45  | 1.50837E+25 | -11.33 | g | 5.45  | 3.09215E+26 | -14.60 | J |
| 6.44  | 9.69888E+24 | -10.85 | g | 6.44  | 1.88057E+26 | -14.06 | J |
| 7.43  | 9.30613E+24 | -10.80 | g | 7.43  | 1.46593E+26 | -13.79 | J |
| 8.42  | 1.06830E+25 | -10.95 | g | 8.42  | 1.04793E+26 | -13.43 | J |
| 9.41  | 9.27390E+24 | -10.80 | g | 9.41  | 7.08431E+25 | -13.00 | J |
| 10.40 | 9.19524E+24 | -10.79 | g | 10.40 | 5.78455E+25 | -12.78 | J |
| 11.39 | 6.29801E+24 | -10.38 | g | 11.39 | 2.97244E+25 | -12.06 | J |
| 0.50  | 1.29382E+27 | -16.16 | r | 0.50  | 8.45222E+26 | -15.70 | H |
| 0.64  | 1.14902E+27 | -16.03 | r | 0.64  | 8.56377E+26 | -15.71 | H |
| 0.99  | 8.50274E+26 | -15.70 | r | 0.99  | 8.76308E+26 | -15.74 | H |
| 1.49  | 6.21757E+26 | -15.36 | r | 1.49  | 6.77426E+26 | -15.46 | H |
| 2.43  | 2.43402E+26 | -14.35 | r | 2.43  | 7.76911E+26 | -15.61 | H |
| 3.47  | 1.17989E+26 | -13.56 | r | 3.47  | 6.38087E+26 | -15.39 | H |
| 4.41  | 6.90316E+25 | -12.98 | r | 4.41  | 5.47101E+26 | -15.22 | H |
| 5.45  | 4.63674E+25 | -12.54 | r | 5.45  | 4.50117E+26 | -15.01 | H |
| 6.44  | 3.02903E+25 | -12.08 | r | 6.44  | 2.97186E+26 | -14.56 | H |
| 7.43  | 2.64714E+25 | -11.94 | r | 7.43  | 2.40051E+26 | -14.33 | H |
| 8.42  | 2.46373E+25 | -11.86 | r | 8.42  | 1.75629E+26 | -13.99 | H |
| 9.41  | 2.04940E+25 | -11.66 | r | 9.41  | 1.23845E+26 | -13.61 | H |
| 10.40 | 1.89003E+25 | -11.57 | r | 10.40 | 9.18316E+25 | -13.29 | H |
| 11.39 | 9.51188E+24 | -10.82 | r | 11.39 | 4.76069E+25 | -12.57 | H |
| 0.50  | 1.27211E+27 | -16.14 | i | 0.50  | 5.27123E+26 | -15.18 | K |
| 0.64  | 1.16239E+27 | -16.04 | i | 0.64  | 5.59925E+26 | -15.25 | K |
| 0.99  | 9.27863E+26 | -15.80 | i | 0.99  | 6.14145E+26 | -15.35 | K |
| 1.49  | 6.69659E+26 | -15.44 | i | 1.49  | 5.53134E+26 | -15.24 | K |
| 2.43  | 3.82166E+26 | -14.83 | i | 2.43  | 6.81496E+26 | -15.46 | K |
| 3.47  | 2.30523E+26 | -14.29 | i | 3.47  | 6.60708E+26 | -15.43 | K |
| 4.41  | 1.63926E+26 | -13.92 | i | 4.41  | 5.87432E+26 | -15.30 | K |
| 5.45  | 1.05893E+26 | -13.44 | i | 5.45  | 6.00685E+26 | -15.33 | K |
| 6.44  | 6.66017E+25 | -12.94 | i | 6.44  | 4.15938E+26 | -14.93 | K |
| 7.43  | 5.15043E+25 | -12.66 | i | 7.43  | 3.94515E+26 | -14.87 | K |
| 8.42  | 3.81874E+25 | -12.33 | i | 8.42  | 3.23483E+26 | -14.65 | K |
| 9.41  | 3.11568E+25 | -12.11 | i | 9.41  | 2.57434E+26 | -14.41 | K |
| 10.40 | 2.54864E+25 | -11.89 | i | 10.40 | 2.02132E+26 | -14.14 | K |
| 11.39 | 1.24449E+25 | -11.12 | i | 11.39 | 1.10890E+26 | -13.49 | K |

## ADDITIONAL REFERENCES

- Berger E., et al., 2007, [ApJ](#), 664, 1000
- Bloom J. S., et al., 2006, [ApJ](#), 638, 354
- Castro-Tirado A. J., et al., 2005, [A&A](#), 439, L15
- D’Avanzo P., et al., 2009, [A&A](#), 498, 711
- Fong W., Berger E., Margutti R., Zauderer B. A., 2015, [ApJ](#), 815, 102
- Fox D. B., et al., 2005, [Nature](#), 437, 845
- Hjorth J., et al., 2005, [ApJ](#), 630, L117
- Jin Z.-P., et al., 2016, [Nature Communications](#), 7, 12898
- Jin Z.-P., et al., 2018, [ApJ](#), 857, 128
- Kasliwal M. M., Korobkin O., Lau R. M., Wollaeger R., Fryer C. L., 2017, [ApJ](#), 843, L34
- Knust F., et al., 2017, [A&A](#), 607, A84
- Kocevski D., et al., 2010, [MNRAS](#), 404, 963
- Malesani D., et al., 2007, [A&A](#), 473, 77
- Nicuesa Guelbenzu A., et al., 2012a, [A&A](#), 538, L7
- Nicuesa Guelbenzu A., et al., 2012b, [A&A](#), 548, A101
- Pérez-Ramírez D., et al., 2013, in Castro-Tirado A. J., Gorosabel J., Park I. H., eds, EAS Publications Series Vol. 61, EAS Publications Series. pp 345–349, [doi:10.1051/eas/1361055](#)
- Rowlinson A., et al., 2010, [MNRAS](#), 409, 531
- Stratta G., et al., 2007, [A&A](#), 474, 827
- Tanvir N. R., Levan A. J., Fruchter A. S., Hjorth J., Hounsell R. A., Wiersema K., Tunnicliffe R. L., 2013, [Nature](#), 500, 547
- Troja E., et al., 2016, [ApJ](#), 827, 102
- Watson D., Hjorth J., Jakobsson P., Xu D., Fynbo J. P. U., Sollerman J., Thöne C. C., Pedersen K., 2006, [A&A](#), 454, L123
